# Supplementary material for: Dual-level Mixup for Graph Few-shot Learning with Fewer Tasks
Source: arXiv:2502.14158 source file (2025-02-19)
Supplement: Supplementary file 1 [file appendix_pre.tex]

\section*{Appendix}
\section{Description of Symbols}
\label{symbol}

\begin{table}[ht]

\centering
\caption{Descriptions of the symbols.}
\label{symbols}
\resizebox{0.5\textwidth}{!}{%
\begin{tabular}{@{}c|c@{}}
\toprule
Symbols & Descriptions \\ \midrule
    $\mathcal{G}, \mathcal{V}, \mathcal{E}$    & Graph, node set, and edge set             \\
    $\mathrm{Z}, \mathrm{A}$    & Initialized node features and adjacency matrix             \\
    $\hat{\mathrm{D}}, \mathrm{H}, \mathrm{X}$    &  Degree matrix, hidden vectors, and refined vectors            \\
    $\kappa, \alpha, \beta$    &   Interaction weights, node centralities, and adjusted scores           \\
    $N, K, M$    & $N$ way, $K$ shot, $M$ query \\
    $\mathcal{D}_{org}$    &   Original meta-training tasks           \\ 
    $\mathcal{D}_{aug}$ & Generated meta-training tasks \\ 
    $\mathcal{D}_{all}$ & All original and generated meta-training tasks  \\
    $\mathcal{S}_t, \mathcal{Q}_t$ & Support and query set \\
    $n_s, n_q$ & Number of samples in $\mathcal{S}_t$ and $\mathcal{Q}_t$ \\
    $\mathcal{T}_{tes}$ & Meta-testing task \\
    $\mathcal{S}_{tes}, \mathcal{Q}_{tes}$ & Support and query set of $\mathcal{T}_{tes}$ \\
    $\eta, \zeta$ & Hyperparameters in Beta distribution \\
    $\lambda$ & Random variable drawn from Beta distribution \\
    $\mathcal{S}_t^\prime, \mathcal{Q}_t^\prime$ & Generated support and query set \\
    $n_{s^\prime}, n_{q^\prime}$ & Number of samples in $\mathcal{S}_t^\prime$ and $\mathcal{Q}_t^\prime$ \\
    $m^\prime, m$ & Number of samples in $\mathcal{S}_t\cup\mathcal{S}_t^\prime$ and $\mathcal{Q}_t\cup\mathcal{Q}_t^\prime$ \\
    $\mathcal{T}_t^{aug}, \tilde{\mathcal{S}}, \tilde{\mathcal{Q}}$ & Interpolated task with its support and query set \\
    $\mathrm{T}_{org}$ & Number of tasks in $\mathcal{D}_{org}$ \\
    $\mathrm{T}_{aug}$ & Number of tasks in $\mathcal{D}_{aug}$ \\
    $\mathrm{T}$ & Number of tasks in $\mathcal{D}_{all}$ \\
    \bottomrule
\end{tabular} %
}
\end{table}

We summarize the used important symbols in Table \ref{symbols}.

\section{Complexity Analysis}
\label{complexity}
We analyze the time complexity of our proposed model to demonstrate its effectiveness. Our model mainly contains two parts, including node presentation learning and dual-level mixup. As linear interpolation is employed in the dual-level mixup, it does not introduce additional time complexity. Basically, most of the time-consuming operations arise from the node embedding process. Here, we choose SGC as the base graph encoder, which removes layer-wise non-linear operations and performs feature extraction in a parameter-free manner. The required time complexity of this step is $O(n^2d)$, where $n$ and $d$ denote the number of nodes and the dimension of node features, respectively. Note that as feature extraction does not require any weights, it is essentially equivalent to a preprocessing step and can be precomputed in practice. Moreover, in the procedure of incorporating degree-based prior information to obtain the refined node representations, the required time complexity is $O(2nd+n)$. Thus, the overall time complexity of our approach is $O(n^2d) + O(2nd+n)$, which is acceptable to us. %compresses layer-wise weights into a learnable matrix, thus involving only a linear transformation operation, while the message aggregation in the GNNs is completed during the preprocessing phase. Therefore, the time complexity required for this step is O(n). The time complexity of 2-layer SGC is $O(ND)$.

\section{Theoretical Proof}
\label{proof}
\subsection{Proof of Eqs.\ref{loss_appro} and \ref{m_theta}}
%Before formally proving Lemma \ref{lemma_first}, let us review some of the adopted notations. After performing intra-task mixup on the original data $\mathcal{D}_{org}=\{\mathcal{T}_{t}\}_{t=1}^{\mathrm{T}_{org}}=\{\{(\mathrm{X}_{t,i}^s,\mathrm{Y}_{t,i}^s)\}_{i=1}^{N^s},\{(\mathrm{X}_{t,i}^q,\mathrm{Y}_{t,i}^q)\}_{i=1}^{N^q}\}\}_{t=1}^{\mathrm{T}_{org}}$, we obtain the interpolated tasks, denoted as $\hat{\mathcal{D}}_{org}=\{\hat{\mathcal{T}}_{t}\}_{t=1}^{\mathrm{T}_{org}}=\{\{(\mathrm{X}_{t,i}^s,\mathrm{Y}_{t,i}^s)\}_{i=1}^{N^s+N^{s^\prime}},\{(\mathrm{X}_{t,i}^q,\mathrm{Y}_{t,i}^q)\}_{i=1}^{N^q+N^{q^\prime}}\}_{t=1}^{\mathrm{T}_{org}}$. Then, we conduct inter-task interpolation on the $\hat{\mathcal{D}}$ to obtain the augmented data $\hat{\mathcal{D}}_{aug}=\{\hat{\mathcal{T}}_t\}_{t=1}^{\mathrm{T}_{aug}}=\{\{(\mathrm{X}_{t,i}^s,\mathrm{Y}_{t,i}^s)\}_{i=1}^{N^s+N^{s^\prime}},\{(\mathrm{X}_{t,i}^q,\mathrm{Y}_{t,i}^q)\}_{i=1}^{N^q+N^{q^\prime}}\}_{t=1}^{\mathrm{T}_{aug}}$. The final training data is composed of original and augmented data, denoted as $\tilde{\mathcal{D}}=\hat{\mathcal{D}}_{org}\cup\hat{\mathcal{D}}_{aug}=\{\hat{\mathcal{T}}\}_{i=1}^\mathrm{T}$. Now, we begin the formal proof.
To prove Eqs.\ref{loss_appro} and \ref{m_theta}, we give the following Lemma \ref{lemma_first}.

\begin{lemma}
\label{lemma_first}
Suppose the designed model with mixup distribution $\lambda \sim \text{Beta}(\eta,\gamma)$. Let $\rho_\lambda \sim \frac{\eta}{\eta\!+\!\gamma}\text{Beta}(\eta\!+\!1,\gamma)\!+\!\frac{\gamma}{\eta\!+\!\gamma}(\gamma\!+\!1,\eta)$. The approximation of the loss function $\mathcal{L}(\mathcal{D}_{all};\theta)$ is given by,
\begin{equation}
    \mathcal{L}(\mathcal{D}_{all};\theta)\approx
    \mathcal{L}(\mathcal{D}_{org};\theta)\!+\!\mathcal{L}(\bar{\lambda}\mathcal{D}_{org};\theta)\!+\!\mathcal{M}(\theta),
\end{equation}
where $\bar{\lambda}\!=\!\mathbb E_{\rho_\lambda}[\lambda]$ and $\mathcal{M}(\theta)$ is a quadratic regularization term with respect to $\theta$, defined as 
\begin{equation}
\begin{aligned}
    \mathcal{M}(\theta)\!=\!\mathbb E_{\mathcal{T}_t\sim p(\mathcal{T})}\mathbb E_{(\mathrm{X}_t,\mathrm{Y}_t)\sim q(\mathcal{T}_t)} \frac{\phi(\mathrm{P}_t)(\phi(\mathrm{P}_t)\!-\!0.5)}{2(1\!+\!\exp{(\mathrm{P}_t)})}(\theta^\top\Sigma_\mathrm{X}\theta)
\end{aligned}
\end{equation}
in which $\mathrm
P_t\!=\!\langle\mathrm{X}_t^q \! - \! (\mathrm{C}_1 \! + \! \mathrm{C}_2)/2,\theta\rangle$, $\phi(\mathrm{P}_t)\!=\!\exp(\mathrm{P}_t)/(1\!+\!\exp(\mathrm{P}_t))$, and $\Sigma_\mathrm{X}\!=\!\mathbb E[\mathrm{X}\mathrm{X}^\top]\!=\!\frac{1}{m}\sum\nolimits_{i=1}^m\mathrm{X}_i\mathrm{X}_i^\top$.
\end{lemma}

\begin{proof}
As stated in Section \ref{theorem_section}, the adopted simplified loss function for binary classification can be formulated as:
\begin{equation}
\label{all}
\begin{aligned}
    &\mathcal{L}(\mathcal{D}_{all};\theta)=\mathcal{L}(\mathcal{D}_{org};\theta) + \mathcal{L}(\mathcal{D}_{aug};\theta) \\
    &= \mathcal{L}(\{\mathcal{T}_t\}_{t=1}^{\mathrm{T}_{org}};\theta) + \mathcal{L}(\{\mathcal{T}_t^{aug}\}_{t=1}^{\mathrm{T}_{aug}};\theta) \\
    &=\mathbb E_{\mathcal{T}_t \sim p(\mathcal{T})} \mathbb E_{(\mathrm{X}_t, \mathrm{Y}_t) \sim q(\mathcal{T}_t)}(1+\exp(\langle\mathrm{X}_{t}^q-(\mathrm{C}_1+\mathrm{C}_2)/2,\theta\rangle))^{-1} + \\
    & \mathbb E_{\mathcal{T}_t^{aug} \sim p(\mathcal{T}^{aug})}\mathbb E_{(\tilde{\mathrm{X}}_t, \tilde{\mathrm{Y}}_t) \sim q(\mathcal{T}_t^{aug})}(1+\exp(\langle\tilde{\mathrm{X}}_{t}^{q}-(\tilde{\mathrm{C}}_1+\tilde{\mathrm{C}}_2)/2,\theta\rangle))^{-1},
\end{aligned}
\end{equation}
where 

\begin{equation}
    \begin{aligned}
        \mathrm{C}_k=\frac{1}{|\mathcal{S}_{t,k}|}\sum_{(\mathrm{X}_{t,i}^s,\mathrm{Y}_{t,i}^s)\in\mathcal{S}_{t}}\mathbb{I}_{\mathrm{Y}_{t,i}=k}\mathrm{X}_{t,i}^s, \\
        \tilde{\mathrm{C}}_k=\frac{1}{|\tilde{\mathcal{S}}_{t,k}|}\sum_{(\tilde{\mathrm{X}}_{t,i}^s,\tilde{\mathrm{Y}}_{t,i}^s)\in\tilde{\mathcal{S}}_{t}}\mathbb{I}_{\tilde{\mathrm{Y}}_{t,i}=k}\tilde{\mathrm{X}}_{t,i}^s.
    \end{aligned}
\end{equation}

Since the preprocessed centralized dataset satisfies the condition $\mathbb E_{\mathcal{T}_t\sim p(\mathcal{T})}\mathbb E_{(\mathrm{X}_t,\mathrm{Y}_t)\sim q(\mathcal{T}_t)}\mathrm{X}_t=\frac{1}{\mathrm{T}_{org}}\sum_{t=1}^{\mathrm{T}_{org}}\frac{1}{2n_q}\sum_{k=1}^2\sum_{i=1}^{n_q}\theta^\top\mathrm{X}_{t,i;k}=0$, which means that the overall sample mean equals 0, we can obtain $\frac{1}{\bar{\lambda}}\mathbb E[\tilde{\mathrm{X}}_{t,i;k}|\mathrm{X}_{t,i;k}]=\mathrm{X}_{t,i;k}$. Moreover, as we simultaneously include linear weights and biases, the predictions are invariant to scaling and shifting of $\tilde{\mathrm{X}}_t$, so it suffices to consider $\{\tilde{\mathrm{X}}_t,\tilde{\mathrm{Y}}_t\}_{t=1}^{\mathrm{T}_{aug}}$ with $\tilde{\mathrm{X}}=\frac{1}{\bar{\lambda}}(\lambda\mathrm{X}_{t;k}+(1-\lambda)\mathrm{X}_{m;k})$. Then, we apply the second-order Taylor expansion on $\mathcal{L}(\mathcal{D}_{aug};\theta) = \mathcal{L}(\{\mathcal{T}_t^{aug}\}_{t=1}^{\mathrm{T}_{aug}};\theta)=\mathbb E_{\mathcal{T}_t^{aug} \sim p(\mathcal{T}^{aug})}\mathbb E_{(\tilde{\mathrm{X}}_t, \tilde{\mathrm{Y}}_t) \sim q(\mathcal{T}_t^{aug})}(1+\exp(\langle\tilde{\mathrm{X}}_{t}^{q}-(\tilde{\mathrm{C}}_1+\tilde{\mathrm{C}}_2)/2,\theta\rangle))^{-1}$ with respect to $\tilde{\mathrm{X}}_{t}^q$ around $\frac{1}{\bar{\lambda}}\mathbb E[\tilde{\mathrm{X}}_{t,i;k}^q|\mathrm{X}_{t,i;k}^q]=\theta^\top\mathrm{X}_{t,i;k}^q$ as follows.
\begin{equation}
    \begin{aligned}
    \label{aug}
        \mathcal{L}(\mathcal{D}_{aug};\theta) &\approx \mathcal{L}(\bar{\lambda}\mathcal{D}_{org};\theta) + \frac{\partial \mathcal{L}({\mathcal{D}_{org}};\theta)}{\partial\theta^\top\mathrm{X}_{t}^q}(\theta^\top\tilde{\mathrm{X}}_t^q-\theta^\top\mathrm{X}_t^q) \\
        &+ (\theta^\top\tilde{\mathrm{X}}_t^q-\theta^\top\mathrm{X}_t^q)^\top\frac{\partial^2 \mathcal{L}({\mathcal{D}_{org};\theta})}{\partial(\theta^\top\mathrm{X}_{t}^q)^2}(\theta^\top\tilde{\mathrm{X}}_t^q-\theta^\top\mathrm{X}_t^q)
    \end{aligned}
\end{equation}
For ease of presentation, let $\mathrm{H}_t=\theta^\top\mathrm{X}_t^q$ and $\mathrm{P}_t=\langle\mathrm{X}_t^q-(\mathrm{C}_1+\mathrm{C}_2)/2,\theta\rangle$. Then, we have 
\begin{equation}
\begin{aligned}
\label{first_order}
    &\frac{\partial \mathcal{L}({\mathcal{D}_{org}};\theta)}{\partial\mathrm{H}_t} = \frac{\partial\mathcal{L}(\mathcal{D}_{org};\theta)}{\partial \mathrm{P}_t} \times \frac{\partial{\mathrm{P}_t}}{\partial \mathrm{H}_t} \\
    &= \mathbb E_{\mathcal{T}_t\sim p(\mathcal{T})}\mathbb E_{(\mathrm{X}_t,\mathrm{Y}_t)\sim q(\mathcal{T}_t)}\frac{\exp(\mathrm{P}_t)}{2(1+\exp(\mathrm{P}_t))^2}
\end{aligned}
\end{equation}
By defining the function $\phi(\mathrm{P}_t)=\frac{\exp(\mathrm{P}_t)}{1+\exp({\mathrm{P}_t})}$, we have
\begin{equation}
\label{second_order}
    \begin{aligned}
        &\frac{\partial^2 \mathcal{L}(\mathcal{D}_{org};\theta)}{\partial \mathrm{H}_t^2} = \mathbb E_{\mathcal{T}_t\sim p(\mathcal{T})}\mathbb E_{(\mathrm{X}_t,\mathrm{Y}_t)\sim q(\mathcal{T}_t)} \\
        &\left[-\frac{\exp{(\mathrm{P}_t)}}{(1+\exp{(\mathrm{P}_t}))^3}\frac{\exp{(\mathrm{P}_t)}}{\partial \mathrm{H}_t} + \frac{1}{2(1+\exp{(\mathrm{P}_t)})^2}\frac{\partial \exp{(\mathrm{P}_t)}}{\partial \mathrm{H}_t} \right] \\
        &= \mathbb E_{\mathcal{T}_t\sim p(\mathcal{T})}\mathbb E_{(\mathrm{X}_t,\mathrm{Y}_t)\sim q(\mathcal{T}_t)} \left[ \frac{\exp{(\mathrm{P}_t)^2}}{2(1+\exp{(\mathrm{P}_t)})^3} - \frac{\exp{(\mathrm{P}_t)}}{4(1+\exp{(\mathrm{P}_t)})^2} \right] \\
        &= \mathbb E_{\mathcal{T}_t\sim p(\mathcal{T})}\mathbb E_{(\mathrm{X}_t,\mathrm{Y}_t)\sim q(\mathcal{T}_t)} \frac{\exp{(\mathrm{P}_t)}(\phi(\mathrm{P}_t)-0.5)}{2(1+\exp{(\mathrm{P}_t)})^2} \\
        &= \mathbb E_{\mathcal{T}_t\sim p(\mathcal{T})}\mathbb E_{(\mathrm{X}_t,\mathrm{Y}_t)\sim q(\mathcal{T}_t)} \frac{\phi(\mathrm{P}_t)(\phi(\mathrm{P}_t)-0.5)}{2(1+\exp{(\mathrm{P}_t)})}
    \end{aligned}
\end{equation}
Plugging Eqs.\ref{first_order} and \ref{second_order} into the Eq.\ref{aug}, we can obtain
\begin{equation}
    \begin{aligned}
    \label{aug_refine}
        &\mathcal{L}(\mathcal{D}_{aug};\theta)\approx \mathcal{L}(\bar{\lambda}\mathcal{D}_{org};\theta) + \\
        & \mathbb E_{\mathcal{T}_t\sim p(\mathcal{T})}\mathbb E_{(\mathrm{X}_t,\mathrm{Y}_t)\sim q(\mathcal{T}_t)}\frac{\exp(\mathrm{P}_t)}{2(1+\exp(\mathrm{P}_t))^2} (\theta^\top\tilde{\mathrm{X}}_t^q-\theta^\top\mathrm{X}_t^q) + \\
        &\Big((\theta^\top\tilde{\mathrm{X}}_t^q-\theta^\top\mathrm{X}_t^q)^\top\mathbb E_{\mathcal{T}_t\sim p(\mathcal{T})}\mathbb E_{(\mathrm{X}_t,\mathrm{Y}_t)\sim q(\mathcal{T}_t)} \\ &\frac{\phi(\mathrm{P}_t)(\phi(\mathrm{P}_t)-0.5)}{2(1+\exp{(\mathrm{P}_t)})}(\theta^\top\tilde{\mathrm{X}}_t^q-\theta^\top\mathrm{X}_t^q)\Big)
    \end{aligned}
\end{equation}

Since $\mathbb E[\tilde{\mathrm{X}}_t - \mathrm{X}_t]=0$ and $\text{Var}(\tilde{\mathrm{X}}_t)=\mathbb E[\mathrm{X}\mathrm{X}^\top]=\Sigma_\mathrm{X}$, the first-order term vanishes and we then simplify the above equation as

\begin{equation}
\begin{aligned}
\label{simplify}
    &\mathcal{L}(\mathcal{D}_{aug};\theta) \approx \mathcal{L}(\bar{\lambda}\mathcal{D}_{org};\theta) \\
    & +  \mathbb E_{\mathcal{T}_t\sim p(\mathcal{T})}\mathbb E_{(\mathrm{X}_t,\mathrm{Y}_t)\sim q(\mathcal{T}_t)} \frac{\phi(\mathrm{P}_t)(\phi(\mathrm{P}_t)-0.5)}{2(1+\exp{(\mathrm{P}_t)})}(\theta^\top\Sigma_\mathrm{X}\theta)
\end{aligned}
\end{equation}

Combining Eqs.\ref{all} and \ref{simplify}, we can acquire
\begin{equation}
    \begin{aligned}
        &\mathcal{L}(\mathcal{D}_{all};\theta) = \mathcal{L}(\mathcal{D}_{org};\theta) + \mathcal{L}(\mathcal{D}_{aug};\theta) \\
        &\approx \mathcal{L}(\mathcal{D}_{org};\theta) + \mathcal{L}(\bar{\lambda}\mathcal{D}_{org};\theta) \\
        & +  \mathbb E_{\mathcal{T}_t\sim p(\mathcal{T})}\mathbb E_{(\mathrm{X}_t,\mathrm{Y}_t)\sim q(\mathcal{T}_t)} \frac{\phi(\mathrm{P}_t)(\phi(\mathrm{P}_t)-0.5)}{2(1+\exp{(\mathrm{P}_t)})}(\theta^\top\Sigma_\mathrm{X}\theta)\\
        &= \mathcal{L}(\mathcal{D}_{org};\theta) + \mathcal{L}(\bar{\lambda}\mathcal{D}_{org};\theta) + \mathcal{M}(\theta)
    \end{aligned}
\end{equation}
Thus, we complete the proof and derive the desired results.
\end{proof}

\subsection{Proof of Theorem \ref{theorem_1}}
Before formally proving Theorem \ref{theorem_1}, we first provide some relevant definitions. The \textit{Rademacher complexity} \cite{mohri2018foundations} reflects the richness of a function class by measuring the extent to which the hypothesis set fits random noise. It is a commonly used and flexible measure of complexity for hypothesis classes, which is defined formally as follows.
\begin{definition}
    \textbf{Empirical Rademacher Complexity}. \textit{The empirical Rademacher complexity of a function class $\mathcal{F}$ with respect to a sample set $\{z_i\}_{i=1}^m$ of size $m$ drawn from a specific data distribution is defined as}:
    \begin{equation}
        \hat{\mathcal{R}}(\mathcal{F}|z_1,\dots,z_m)=\underset{\sigma}{\mathbb{E}}\left[\underset{f\in\mathcal{F}}{\text{sup}}\frac{1}{m}\sum_{i=1}^m\sigma_if(z_i)\right],
    \end{equation}
\textit{where $\sigma=[\sigma_1,\dots,\sigma_m]^\top$ are Rademacher variables, in which $\sigma_i$ follows a uniform distribution and takes values in $\{-1,+1\}$}.
\end{definition}

Next, we present the definition of \textit{Rademacher complexity}, which eliminates the dependence on specific sample sets and provides a more uniform measure of the complexity of a function class.

\begin{definition}
    \textbf{Rademacher Complexity}. \textit{The Rademacher complexity of a function class $\mathcal{F}$} is defined by the expectation of the empirical Rademacher complexity over all samples of size $m$ drawn according to data distribution $\mathbb{P}$:
    \begin{equation}
        \mathcal{R}(\mathcal{F})=\underset{\{z_1,\dots,z_m\}\sim \mathbb{P}}{\mathbb{E}}\hat{\mathcal{R}}(\mathcal{F}|z_1,\dots,z_m).
    \end{equation}
\end{definition}

The \textit{integral probability metric} \cite{muller1997integral} is a type of distance function between probability distributions that measures how a class of functions distinguishes between two probability distributions. Its formal definition is as follows.
\begin{definition}
    \textbf{Integral Probability Metric}. \textit{The integral probability metric between two probability distributions $\mathbb{P}$ and $\mathbb{Q}$ on the data space $\mathcal{Z}$ with respect to the class of real-valued bounded measurable functions $\mathcal{F}$ is given by}:
    \begin{equation}
        \mathcal{D}_\mathcal{F}(\mathbb{P},\mathbb{Q})=\underset{f\in\mathcal{F}}{\text{sup}}\left|\mathbb{E}_\mathbb{P}f(\mathcal{Z})-\mathbb{E}_\mathbb{Q}f(\mathcal{Z})\right|.
    \end{equation}
\end{definition}

Next, we present the standard uniform deviation bound in Lemma \ref{lemma_1} \cite{mohri2018foundations} using Rademacher complexity.
\begin{lemma}
\label{lemma_1}
    Let $\mathcal{F}$ be a collection of functions mapping from $\mathcal{Z}$ to $[a,a+1]$. For $\epsilon > 0$, with probability at least $(1-\epsilon)$ over an i.i.d. sample set $\{z_i\}_{i=1}^m$ drawn from a distribution $\mathbb{P}$ over $\mathcal{Z}$, each $f$ in $\mathcal{F}$ satisfies:
    \begin{equation}
    \label{sud}
    \begin{aligned}
        &\mathbb{E}_{\mathbb{P}}f(z)\leq\frac{1}{m}\sum_{i=1}^mf(z_i)+2\mathcal{R}(\mathcal{F})+\sqrt{\frac{\log(1/\epsilon)}{2m}},\;\text{or} \\
        &\mathbb{E}_{\mathbb{P}}f(z)\leq\frac{1}{m}\sum_{i=1}^mf(z_i)+2\hat{\mathcal{R}}(\mathcal{F}|z_1,\cdots,z_m)+3\sqrt{\frac{\log(2/\epsilon)}{2m}},
    \end{aligned} 
    \end{equation}
    where $\mathcal{R}(\mathcal{F})$ and $\hat{\mathcal{R}}(\mathcal{F}|z_1,\cdots,z_m)$ are the Rademacher complexity and the empirical Rademacher complexity, respectively.
\end{lemma}
We can leverage the integral probability metric to transform Eq.\ref{sud} into the following form:
\begin{equation}
\begin{aligned}
    \mathcal{D}_\mathcal{F}(\hat{\mathbb{P}},\mathbb{P}) &= \underset{f\in\mathcal{F}}{\text{sup}}\left|\mathbb{E}_{\hat{\mathbb{P}}}f(z)-\mathbb{E}_{\mathbb{P}}f(z)\right|\leq2\mathcal{R}(\mathcal{F})+\sqrt{\frac{\log(1/\epsilon)}{2m}}, or\\
    \mathcal{D}_\mathcal{F}(\hat{\mathbb{P}},\mathbb{P}) &= \underset{f\in\mathcal{F}}{\text{sup}}\left|\mathbb{E}_{\hat{\mathbb{P}}}f(z)-\mathbb{E}_{\mathbb{P}}f(z)\right|\leq2\hat{\mathcal{R}}(\mathcal{F}|z_1,\cdots,z_m)+3\sqrt{\frac{\log(2/\epsilon)}{2m}},
\end{aligned}
\end{equation}
where $\hat{\mathbb{P}}$ denotes the empirical distribution of samples.

Additionally, we introduce Lemma \ref{lemma_2} that bounds the Rademacher complexity, which is utilized in the proof of Theorem \ref{theorem_1}.
\begin{lemma}
\label{lemma_2}
    %Assume that the distribution of $\mathrm{X}$ is $\tau-$retentive for $\tau \in (0, 1/2]$. 
    Let $\sum_\mathrm{X}=\mathbb{E}[\mathrm{X}\mathrm{X}^\top]$ %$\sum_\mathrm{X}=\mathbb{E}_{\mathcal{T}\sim p(\mathcal{T})}\mathbb{E}_\mathcal{T}[\mathrm{X}\mathrm{X}^\top]$ 
    and $\mathcal{F}_\nu=\{\mathrm{X}\rightarrow\theta^\top \mathrm{X}:%\mathbb{E}_\mathrm{X}[\phi(\left\langle\mathrm{X}-(\mathrm{c}_1+\mathrm{c}_2)/2,\theta\right\rangle)]
    \theta^\top\sum_\mathrm{X}\theta\leq\nu\}$. Then, the Rademacher complexity of $\mathcal{F}_\nu$ satisfies
    \begin{equation}
        \mathcal{R}(\mathcal{F}_\nu)\leq \sqrt{\frac{\nu\cdot\textrm{rank}(\sum_\mathrm{X})}{m}}.
    \end{equation}
\end{lemma}

\begin{proof}
    According to the definition of empirical Rademacher complexity, given a set of \textit{i.i.d} Rademacher random variables, we have:
    \begin{equation*}
    \begin{aligned}
        \hat{\mathcal{R}}(\mathcal{F}|\mathrm{X}_1,\dots,\mathrm{X}_m)&=\underset{\sigma}{\mathbb{E}}\left[\underset{f\in\mathcal{F}}{\text{sup}}\frac{1}{m}\sum_{i=1}^m\sigma_if(\mathrm{X}_i)\right] \\
        &=\underset{\sigma}{\mathbb{E}}\left[\underset{\theta^\top\sum_\mathrm{X}\theta\leq\nu}{\text{sup}}\frac{1}{m}\sum_{i=1}^m\sigma_if(\mathrm{X}_i)\right] \\
        &=\underset{\sigma}{\mathbb{E}}\left[\underset{\theta^\top\sum_\mathrm{X}\theta\leq\nu}{\text{sup}}\frac{1}{m}\sum_{i=1}^m\sigma_i\theta^\top\mathrm{X}_i\right] \\
        &=\underset{\sigma}{\mathbb{E}}\left[\underset{||\Sigma_{\mathrm{X}}^{1/2}\theta||^2\leq \nu}{\text{sup}}\frac{1}{m}\sum_{i=1}^m\sigma_i(\Sigma_{\mathrm{X}}^{1/2}\theta)^\top(\Sigma_{\mathrm{X}}^{\dagger/2}\mathrm{X}_i)\right] \\
        & \leq \frac{\sqrt{\nu}}{m}\underset{\sigma}{\mathbb{E}}\left\Vert\sum_{i=1}^m\sigma_i\Sigma_{\mathrm{X}}^{\dagger/2}\mathrm{X}_i\right\Vert \\
        % &=\frac{\sqrt{\nu}}{m}\left\Vert\sum_{i=1}^m\sigma_i\Sigma_{\mathrm{X}}^{\dagger/2}\mathrm{X}_i\right\Vert_2 \\
        &\leq \frac{\sqrt{\nu}}{m}\sqrt{\underset{\sigma}{\mathbb E}\left\Vert\sum_{i=1}^m\sigma_i\Sigma_{\mathrm{X}}^{\dagger/2}\mathrm{X}_i\right\Vert^{2}} \\
        &\leq \frac{\sqrt{\nu}}{m}\sqrt{\sum_{i=1}^m{(\Sigma_{\mathrm{X}}^{\dagger/2}\mathrm{X}_i)}^\top(\Sigma_{\mathrm{X}}^{\dagger/2}\mathrm{X}_i)} \\
        &= \frac{\sqrt{\nu}}{m} \sqrt{\sum_{i=1}^m\mathrm{X}_i^\top\mathrm{X}_i}\ ,
        %\mathcal{R}(\mathcal{F})=\underset{\{\mathrm{X}_1,\dots,\mathrm{X}_m\}\sim \mathbb{P}}{\mathbb{E}}\hat{\mathcal{R}}(\mathcal{F}|\mathrm{X}_1,\dots,\mathrm{X}_m) \leq \frac{\sqrt{\nu}}{m}\sqrt{\sum_{i=1}^m\mathbb{E}_{\mathrm{X}_i}}
    \end{aligned}
    \end{equation*}
    where $\Sigma_\mathrm{X}^{\dagger}$ is the generalized inverse of $\Sigma_\mathrm{X}$. 
    \begin{equation*}
    \begin{aligned}
        \mathcal{R}(\mathcal{F})&=\underset{\{\mathrm{X}_1,\dots,\mathrm{X}_m\}\sim \mathbb{P}}{\mathbb{E}}\hat{\mathcal{R}}(\mathcal{F}|\mathrm{X}_1,\dots,\mathrm{X}_m) \\ &\leq \frac{\sqrt{\nu}}{m}\sqrt{\sum_{i=1}^m\mathbb{E}_{\mathrm{X}_i}(\mathrm{X}_i^\top\mathrm{X}_i)} \\
        &\leq \frac{\sqrt{\nu}\sqrt{\text{rank}(\Sigma_{\mathrm{X}_i})}}{\sqrt{m}}.
    \end{aligned}
    \end{equation*}
    %where $\Sigma^\dagger$ is the Moore–Penrose inverse of $\Sigma$.
\end{proof}

Now, we are ready to prove the Theorem \ref{theorem_1}.
\begin{proof}
\begin{equation}
\label{risk}
\begin{aligned}
    &|\hat{\mathsf{R}}-\mathsf{R}|\\
    &=\Big|\mathbb E_{\mathcal{T}_i\sim \hat{p}(\mathcal{T})}\mathbb E_{(\mathrm{X}_j,\mathrm{Y}_j)\sim \hat{q}(\mathcal{T}_i)}\mathcal{L}(f_\theta(\mathrm{X}_j),\mathrm{Y}_j)- \\
    & \quad \; \mathbb E_{\mathcal{T}_i\sim p(\mathcal{T})}\mathbb E_{(\mathrm{X}_j,\mathrm{Y}_j)\sim q(\mathcal{T}_i)}\mathcal{L}(f_\theta(\mathrm{X}_j),\mathrm{Y}_j)\Big|\\
    &=\Big|\mathbb E_{\mathcal{T}_i\sim \hat{p}(\mathcal{T})}\mathbb E_{(\mathrm{X}_j,\mathrm{Y}_j)\sim \hat{q}(\mathcal{T}_i)}\mathcal{L}(f_\theta(\mathrm{X}_j),\mathrm{Y}_j) - \\
    & \quad \; \mathbb E_{\mathcal{T}_i\sim \hat{p}(\mathcal{T})}\mathbb E_{(\mathrm{X}_j,\mathrm{Y}_j)\sim q(\mathcal{T}_i)}\mathcal{L}(f_\theta(\mathrm{X}_j),\mathrm{Y}_j) + \\
    & \quad \; \mathbb E_{\mathcal{T}_i\sim \hat{p}(\mathcal{T})}\mathbb E_{(\mathrm{X}_j,\mathrm{Y}_j)\sim q(\mathcal{T}_i)}\mathcal{L}(f_\theta(\mathrm{X}_j),\mathrm{Y}_j) - \\
    & \quad \; \mathbb E_{\mathcal{T}_i\sim p(\mathcal{T})}\mathbb E_{(\mathrm{X}_j,\mathrm{Y}_j)\sim q(\mathcal{T}_i)}\mathcal{L}(f_\theta(\mathrm{X}_j),\mathrm{Y}_j) \Big|
    \end{aligned}
\end{equation}
For the \textit{first two terms} of Eq.\ref{risk}, we can rewrite them as:
\begin{equation}
\label{first_term}
\begin{aligned}
    &\mathbb E_{\mathcal{T}_i\sim \hat{p}(\mathcal{T})} \mathbb E_{(\mathrm{X}_j,\mathrm{Y}_j)\sim \hat{q}(\mathcal{T}_i)}\mathcal{L}(f_\theta(\mathrm{X}_j),\mathrm{Y}_j) - \\
    &\mathbb E_{\mathcal{T}_i\sim \hat{p}(\mathcal{T})}\mathbb E_{(\mathrm{X}_j,\mathrm{Y}_j)\sim q(\mathcal{T}_i)}\mathcal{L}(f_\theta(\mathrm{X}_j),\mathrm{Y}_j) \\
    &\leq \mathbb E_{\mathcal{T}_i\sim \hat{p}(\mathcal{T})}\Big[\mathbb E_{(\mathrm{X}_j,\mathrm{Y}_j)\sim \hat{q}(\mathcal{T}_i)}\mathcal{L}(f_\theta(\mathrm{X}_j),\mathrm{Y}_j) - \\
    & \qquad \qquad \qquad \mathbb E_{(\mathrm{X}_j,\mathrm{Y}_j)\sim q(\mathcal{T}_i)}\mathcal{L}(f_\theta(\mathrm{X}_j),\mathrm{Y}_j)\Big] \\
    &\overset{(i)}{\leq} \mathbb E_{\mathcal{T}_i\sim \hat{p}(\mathcal{T})}[\mathcal{D}_\mathcal{F}(\hat{q},q)] \\
    &\overset{(ii)}{=} \mathbb E_{\mathcal{T}_i\sim \hat{p}(\mathcal{T})}\left[\underset{f\in\mathcal{F}}{\text{sup}}\left|\mathbb{E}_{\hat{q}}\mathcal{L}(f_\theta(\mathrm{X}_j),\mathrm{Y}_j) - \mathbb E_q\mathcal{L}(f_\theta(\mathrm{X}_j),\mathrm{Y}_j)\right|\right] \\
    &\overset{(iii)}{\leq} \mathbb E_{\mathcal{T}_i\sim \hat{p}(\mathcal{T})} \left[2\hat{\mathcal{R}}(\mathcal{F}|\mathrm{X}_1,\cdots,\mathrm{X}_m)+3\sqrt{\frac{\log(2/\epsilon)}{2m}}\right] \\
    &\overset{(iv)}{=}2\mathcal{R}(\mathcal{F}) + 3\sqrt{\frac{\log(2/\epsilon)}{2m}} \\
    %&\overset{(v)}{=} \mathbb E_{\mathcal{T}_i\sim \hat{p}(\mathcal{T})} \left[ 2\sqrt{\frac{\nu\cdot\textrm{rank}(\sum_\mathrm{X})}{m}} + \sqrt{\frac{(b-a)^2\log(1/\epsilon)}{2m}}\right] \\
    &\overset{(v)}{\leq}2\sqrt{\frac{\nu\cdot\textrm{rank}(\sum_\mathrm{X})}{m}} + 3\sqrt{\frac{\log(2/\epsilon)}{2m}},
\end{aligned}
\end{equation}
where Inequality $(i)$ holds due to the definition of the integral probability metric, Equation $(ii)$ is the expansion of the integral probability metric, Inequality $(iii)$ holds due to Lemma \ref{lemma_1}, Equation $(iv)$ is the definition of Rademacher complexity, and Inequality $(v)$ holds due to Lemma \ref{lemma_2}.

For the \textit{last two terms} of Eq.\ref{risk}, we first define a function class $\mathcal{H}$, which satisfies:
\begin{equation*}
\begin{aligned}
    &\mathcal{H}=\{h(\mathcal{T}):h(\mathcal{T})=\mathbb E_{(\mathrm{X}_j,\mathrm{Y}_j)\sim q(\mathcal{T})}(\mathcal{L}(f_\theta(\mathrm{X}_j),\mathrm{Y}_j), \\ &\text{such that}\; f_\theta \in \mathcal{F}_\nu \;\text{and}\; h(\cdot)\; \text{maps}\; \mathcal{T}\; \text{to}\; \mathbb{R}\}.
\end{aligned}
\end{equation*}
Then, by utilizing the integral probability metric and Lemma \ref{lemma_1}, we have
\begin{equation}
\begin{aligned}
    &\mathbb E_{\mathcal{T}_i\sim \hat{p}(\mathcal{T})}\mathbb E_{(\mathrm{X}_j,\mathrm{Y}_j)\sim q(\mathcal{T}_i)}\mathcal{L}(f_\theta(\mathrm{X}_j),\mathrm{Y}_j) - \\
    &\mathbb E_{\mathcal{T}_i\sim p(\mathcal{T})}\mathbb E_{(\mathrm{X}_j,\mathrm{Y}_j)\sim q(\mathcal{T}_i)}\mathcal{L}(f_\theta(\mathrm{X}_j),\mathrm{Y}_j) \\
    &=\mathbb E_{\mathcal{T}_i\sim \hat{p}(\mathcal{T})}h(\mathcal{T}_i) - \mathbb E_{\mathcal{T}_i\sim p(\mathcal{T})}h(\mathcal{T}_i) \\ 
    &= \mathcal{D}_{\mathcal{H}}(\hat{p},p) \\
    &=\underset{h\in\mathcal{H}}{\text{sup}}\left|\mathbb E_{\hat{p}}h(\mathcal{T}_i) - \mathbb E_{p} h(\mathcal{T}_i)\right| \\
    &\leq 2\hat{\mathcal{R}}(\mathcal{H}|\mathcal{T}_1,\cdots,\mathcal{T}_\mathrm{T}) + 3\sqrt{\frac{\log(2/\epsilon)}{2\mathrm{T}}}.
\end{aligned}
\end{equation}
Next, we need to obtain the empirical Rademacher complexity for the defined function class over distributions. According to the definition, we have
\begin{equation}
\label{lad}
\begin{aligned}
    &\hat{\mathcal{R}}(\mathcal{H}|\mathcal{T}_1,\cdots,\mathcal{T}_\mathrm{T}) = \underset{\sigma}{\mathbb E} \left[\underset{h\in\mathcal{H}}{\text{sup}}\frac{1}{\mathrm{T}}\sum_{i=1}^\mathrm{T}\sigma_ih(\mathcal{T}_i)\right]\\
    &=\underset{\sigma}{\mathbb E} \left[\underset{h\in\mathcal{H}}{\text{sup}}\frac{1}{\mathrm{T}}\sum_{i=1}^\mathrm{T}\sigma_i \mathbb E_{(\mathrm{X}_j,\mathrm{Y}_j) \sim q(\mathcal{T}_i)}\left(\frac{1}{1+\exp{(\theta^\top\mathrm{X}_j)}}-\theta^\top\mathrm{X}_j\mathrm{Y}_j\right)\right] \\
    &\leq \underset{\sigma}{\mathbb E} \left[\underset{h\in\mathcal{H}}{\text{sup}}\frac{1}{\mathrm{T}}\sum_{i=1}^\mathrm{T}\sigma_i \mathbb E_{(\mathrm{X}_j,\mathrm{Y}_j) \sim q(\mathcal{T}_i)}\left({\theta^\top\mathrm{X}_t}\right)\right] + \\ 
    & \quad \underset{\sigma}{\mathbb E} \left[\underset{h\in\mathcal{H}}{\text{sup}}\frac{1}{\mathrm{T}}\sum_{i=1}^\mathrm{T}\sigma_i \mathbb E_{(\mathrm{X}_j,\mathrm{Y}_j) \sim q(\mathcal{T}_i)}\left(\theta^\top\mathrm{X}_j\mathrm{Y}_j\right)\right]\\
    &\leq \underbrace{\underset{\sigma}{\mathbb E} \left[\underset{h\in\mathcal{H}}{\text{sup}}\frac{1}{\mathrm{T}}\sum_{i=1}^\mathrm{T}\sigma_i (\Sigma_{\mathrm{X}}^{1/2}\theta)^\top\Sigma_\mathrm{X}^{\dagger/2}\mu_{\mathrm{X}}\right]}_{(i)} + \\ 
    &\underbrace{\underset{\sigma}{\mathbb E} \left[\underset{h\in\mathcal{H}}{\text{sup}}\frac{1}{\mathrm{T}}(\Sigma_\mathrm{X}^{1/2}\theta)^\top\sum_{i=1}^\mathrm{T}\sigma_i \mathbb E_{(\mathrm{X}_j,\mathrm{Y}_j) \sim q(\mathcal{T}_i)} \left(\Sigma_\mathrm{X}^{\dagger/2}\mathrm{X}_j\mathrm{Y}_j\right)\right]}_{(ii)}, \\
\end{aligned}
\end{equation}
where $\mu_\mathrm{X}=\mathbb E_{(\mathrm{X}_j,\mathrm{Y}_j)\sim q(\mathcal{T}_i)}\mathrm{X}_j$.

For the \textit{first term (i)} in Eq.\ref{lad}, we can bound it as follows:
\begin{equation}
\label{lad_first}
    \begin{aligned}    
    &\underset{\sigma}{\mathbb E} \left[\underset{h\in\mathcal{H}}{\text{sup}}\frac{1}{\mathrm{T}}\sum_{i=1}^\mathrm{T}\sigma_i (\Sigma_{\mathrm{X}}^{1/2}\theta)^\top\Sigma_\mathrm{X}^{\dagger/2}\mu_{\mathrm{X}}\right] \\
    &\leq \left\Vert(\Sigma_{\mathrm{X}}^{1/2}\theta)^\top\right\Vert \cdot \underset{\sigma}{\mathbb E}\left[\underset{h\in\mathcal{H}}{\text{sup}}\frac{1}{\mathrm{T}}\sum_{i=1}^\mathrm{T}\sigma_i\Sigma_\mathrm{X}^{\dagger/2}\mu_{\mathrm{X}}\right] \\
    &\leq \sqrt{\nu} \underset{\sigma}{\mathbb E}\left\Vert \frac{1}{\mathrm{T}}\sum_{i=1}^\mathrm{T}\sigma_i\Sigma_\mathrm{X}^{\dagger/2}\mu_{\mathrm{X}}\right\Vert \leq \frac{\sqrt{\nu}}{\mathrm{T}}\sqrt{\underset{\sigma}{\mathbb E}\left\Vert \sum_{i=1}^\mathrm{T}\sigma_i\Sigma_\mathrm{X}^{\dagger/2}\mu_\mathrm{X}\right\Vert^2} \\
    &\leq \frac{\sqrt{\nu}}{\sqrt{\mathrm T}}\left\Vert\Sigma_\mathrm{X}^{\dagger/2}\mu_\mathrm{X}\right\Vert.
\end{aligned}
\end{equation}

For the \textit{second term (ii)} in Eq.\ref{lad}, we have the following bound as follows:
\begin{equation}
\label{lad_second}
    \begin{aligned}
        &\underset{\sigma}{\mathbb E} \left[\underset{h\in\mathcal{H}}{\text{sup}}\frac{1}{\mathrm{T}}(\Sigma_\mathrm{X}^{1/2}\theta)^\top\sum_{i=1}^\mathrm{T}\sigma_i \mathbb E_{(\mathrm{X}_j,\mathrm{Y}_j) \sim q(\mathcal{T}_i)} \left(\Sigma_\mathrm{X}^{\dagger/2}\mathrm{X}_j\mathrm{Y}_j\right)\right] \\
        &\leq \left\Vert(\Sigma_{\mathrm{X}}^{1/2}\theta)^\top\right\Vert \cdot \underset{\sigma}{\mathbb E} \left[\underset{h\in\mathcal{H}}{\text{sup}}\frac{1}{\mathrm{T}}\sum_{i=1}^\mathrm{T}\sigma_i \mathbb E_{(\mathrm{X}_j,\mathrm{Y}_j) \sim q(\mathcal{T}_i)} \left(\Sigma_\mathrm{X}^{\dagger/2}\mathrm{X}_j\mathrm{Y}_j\right)\right] \\
        &\leq \sqrt{\nu}\underset{\sigma}{\mathbb E} \left\Vert\frac{1}{\mathrm{T}}\sum_{i=1}^\mathrm{T}\sigma_i \mathbb E_{(\mathrm{X}_j,\mathrm{Y}_j) \sim q(\mathcal{T}_i)} \left(\Sigma_\mathrm{X}^{\dagger/2}\mathrm{X}_j\mathrm{Y}_j\right)\right\Vert \\
        %&\leq \frac{\sqrt{\nu}}{\mathrm{T}}\underset{\sigma}{\mathbb E}\sqrt{\left\Vert\sum_{i=1}^\mathrm{T}\sigma_i\mathbb E_{(\mathrm{X}_j,\mathrm{Y}_j)\sim q(\mathcal{T}_i)}(\Sigma_\mathrm{X}^{\dagger/2}\mathrm{X}_j\mathrm{Y}_j)\right\Vert^2} \\
        &\leq \frac{\sqrt{\nu}}{\mathrm{T}}\sqrt{\underset{\sigma}{\mathbb E}\left\Vert\sum_{i=1}^\mathrm{T}\sigma_i\mathbb E_{(\mathrm{X}_j,\mathrm{Y}_j)\sim q(\mathcal{T}_i)}(\Sigma_\mathrm{X}^{\dagger/2}\mathrm{X}_j\mathrm{Y}_j)\right\Vert^2} \\
        &\leq \frac{\sqrt{\nu}}{\sqrt{\mathrm{T}}}\sqrt{\sum_{i=1}^\mathrm{T}\mathbb E_{(\mathrm{X}_j,\mathrm{Y}_j)\sim q(\mathcal{T}_i)}\left[(\Sigma_\mathrm{X}^{\dagger/2}\mathrm{X}_j\mathrm{Y}_j)^\top(\Sigma_\mathrm{X}^{\dagger/2}\mathrm{X}_j\mathrm{Y}_j)\right]} \\
        &\leq \frac{\sqrt{\nu}\cdot\text{rank}(\Sigma_\mathrm{X})}{\sqrt{\mathrm{T}}}.
    \end{aligned}
\end{equation}
By combining the derivations from Eqs.\ref{lad_first} and \ref{lad_second}, we have the following bound in Eq.\ref{lad}:
\begin{equation}
    \hat{\mathcal{R}}(\mathcal{H}|\mathcal{T}_1,\cdots,\mathcal{T}_\mathrm{T}) \leq \sqrt{\frac{\nu}{\mathrm{T}}}\left(\left\Vert\Sigma_\mathrm{X}^{\dagger/2}\mu_\mathrm{X}\right\Vert + \text{rank}(\Sigma_\mathrm{X})\right).
\end{equation}
Thus, the last two terms of Eq.\ref{risk} can be bounded as follows:
\begin{equation}
\label{last_term}
    \begin{aligned}
            &\mathbb E_{\mathcal{T}_i\sim \hat{p}(\mathcal{T})}\mathbb E_{(\mathrm{X}_j,\mathrm{Y}_j)\sim q(\mathcal{T}_i)}\mathcal{L}(f_\theta(\mathrm{X}_j),\mathrm{Y}_j) - \\ 
            & \qquad \qquad \mathbb E_{\mathcal{T}_i\sim p(\mathcal{T})}\mathbb E_{(\mathrm{X}_j,\mathrm{Y}_j)\sim q(\mathcal{T}_i)}\mathcal{L}(f_\theta(\mathrm{X}_j),\mathrm{Y}_j) \\
            &\leq 2\hat{\mathcal{R}}(\mathcal{H}|\mathcal{T}_1,\cdots,\mathcal{T}_\mathrm{T}) + 3\sqrt{\frac{\log(2/\epsilon)}{2\mathrm{T}}} \\
            & \leq  2\sqrt{\frac{\nu}{\mathrm{T}}} \left(\left\Vert\Sigma_\mathrm{X}^{\dagger/2}\mu_\mathrm{X}\right\Vert + \text{rank}(\Sigma_\mathrm{X})\right) + 3\sqrt{\frac{\log(2/\epsilon)}{2\mathrm{T}}}.
    \end{aligned}
\end{equation}
By combining the results from Eqs.\ref{first_term} and \ref{last_term}, we can obtain the following result.
\begin{equation}
\begin{aligned}
    &|\hat{\mathsf{R}}-\mathsf{R}|\leq 2\left(\sqrt{\frac{\nu\cdot\textrm{rank}(\sum_\mathrm{X})}{m}} + \sqrt{\frac{\nu}{\mathrm{T}}}\left(\left\Vert\Sigma_\mathrm{X}^{\dagger/2}\mu_\mathrm{X}\right\Vert + \textrm{rank}(\Sigma_\mathrm{X}) \right) \right) + \\ & \qquad \qquad 3\left(\sqrt{\frac{\log(2/\epsilon)}{2m}}+\sqrt{\frac{\log(2/\epsilon)}{2\mathrm{T}}}\right).
\end{aligned}
\end{equation}
When $\mu_\mathrm{X}$ is set to 0, we can obtain the desired outcome as shown in Theorem \ref{theorem_1}, which is listed below.
\begin{equation}
\begin{aligned}
    &|\hat{\mathsf{R}}-\mathsf{R}|\leq 2\left(\sqrt{\frac{\nu\cdot\textrm{rank}(\sum_\mathrm{X})}{m}} + \sqrt{\frac{\nu}{\mathrm{T}}}\left(\textrm{rank}(\Sigma_\mathrm{X}) \right) \right) + \\ & \qquad \qquad 3\left(\sqrt{\frac{\log(2/\epsilon)}{2m}}+\sqrt{\frac{\log(2/\epsilon)}{2\mathrm{T}}}\right).
\end{aligned}
\end{equation}
\end{proof}

\subsection{Proof of Corollary \ref{corollary_1}}
\begin{proof}
According to Theorem \ref{theorem_1}, the upper bound of the model using our proposed strategy can be represented as:
\begin{equation}
\begin{aligned}
    \mathsf{U}(|\hat{\mathsf R}-\mathsf R|) &= 2\left(\sqrt{\frac{\nu\cdot\textrm{rank}(\sum_\mathrm{X})}{m}} + \sqrt{\frac{\nu}{\mathrm{T}}}\left(\textrm{rank}(\Sigma_\mathrm{X}) \right) \right) + \\
    & \quad \; 3\left(\sqrt{\frac{\log(2/\epsilon)}{2m}}+\sqrt{\frac{\log(2/\epsilon)}{2\mathrm{T}}}\right).
\end{aligned}
\end{equation}

The upper bound of the model without any strategy can be represented as:
\begin{equation}
\begin{aligned}
\mathsf{U}(|\hat{\mathsf{R}}_\text{ori}-\mathsf R_\text{ori}|) &= 2\left(\sqrt{\frac{\nu\cdot\textrm{rank}(\sum_\mathrm{X})}{m_\text{ori}}} + \sqrt{\frac{\nu}{\mathrm{T}_\text{ori}}}\left(\textrm{rank}(\Sigma_\mathrm{X}) \right) \right) + \\ & \quad \; 3\left(\sqrt{\frac{\log(2/\epsilon)}{2m_\text{ori}}}+\sqrt{\frac{\log(2/\epsilon)}{2\mathrm{T}_\text{ori}}}\right).
\end{aligned}
\end{equation}
Thus, we can proceed with the proof as follows:

\begin{equation}
\begin{aligned}
    &\mathsf{U}(|\hat{\mathsf R}-\mathsf R|)-\mathsf{U}(|\hat{\mathsf{R}}_\text{ori}-\mathsf R_\text{ori}|) \\
    &=2\left[\sqrt{\nu\cdot\textrm{rank}(\Sigma_\mathrm{X})} \left(\underbrace{\sqrt{\frac{1}{m}} - \sqrt{\frac{1}{m_\text{ori}}}}_{(i)}\right) + \right.\\
    & \qquad \qquad \left. \left( \sqrt{\nu}\left(\text{rank}(\Sigma_\mathrm{X})\right) \left( \underbrace{\sqrt{\frac{1}{\mathrm{T}}}-\sqrt{\frac{1}{\mathrm{T}_\text{ori}}}\mathrm{T}_\text{ori}}_{(ii)}\right)\right) \right] \\
    &+3\left[ \sqrt{\log(2/\epsilon)} \left( \underbrace{ \sqrt{\frac{1}{2m}} - \sqrt{\frac{1}{2m_\text{ori}}}}_{(iii)} \right) + \sqrt{\log(2/\epsilon)}\left( \underbrace{ \sqrt{\frac{1}{2\mathrm{T}}} - \sqrt{\frac{1}{2\mathrm{T}_\text{ori}}}}_{(iv)} \right) \right].
\end{aligned}
\end{equation}

Due to the introduction of within-task interpolation, we have $m > m_\text{ori}$, thus inequalities $(i)$ and $(iii)$ are both less than 0. Furthermore, due to the introduction of inter-task interpolation, we have $T > T_\text{ori}$, thus inequalities $(ii)$ and $(iv)$ are also both less than 0. Therefore, the inequality $\mathsf{U}(|\hat{\mathsf R}-\mathsf R|) \leq \mathsf{U}(|\hat{\mathsf R}_\text{ori}-\mathsf R_\text{ori}|)$ is held. The Corollary \ref{corollary_1} is also satisfied.
\end{proof}

\subsection{Proof of Theorem \ref{theorem_2}}
%In fact, the goal of meta-learning is to reduce the distance between the training data distribution and the testing data distribution through the model learning. We formally state the relevant theorem as follows.
According to Theorem \ref{theorem_2}, we have
\begin{equation}
    \underset{f\in\mathcal{F}}{\text{sup}}|\mathbb{E}_{\hat{\mathbb P} }-\mathbb E_{\mathbb Q}| \leq \left(2\sqrt{\nu\cdot\text{rank}(\Sigma_{\mathrm{X}})} + \sqrt{\frac{\log(1/\epsilon)}{2}} \right) \left( \sqrt{\frac{1}{m}} + \sqrt{\frac{1}{n_q}} \right).
\end{equation}
The procedure of Theorem \ref{theorem_2} is summarized as follows.
\begin{proof}
\begin{equation}
\label{ipm}
    \begin{aligned}
        \underset{f\in\mathcal{F}}{\text{sup}} |\mathbb{E}_{\hat{\mathbb P} }-\mathbb E_{\mathbb Q}| &= \underset{f\in\mathcal{F}}{\text{sup}}|\mathbb{E}_{\hat{\mathbb P} } - \mathbb E_{\hat{\mathbb Q}} + \mathbb E_{\hat{\mathbb Q}} - \mathbb E_{\mathbb Q}| \\
        &\leq \underset{f\in\mathcal{F}}{\text{sup}} \left[ \left|\mathbb{E}_{\hat{\mathbb P} } - \mathbb E_{\hat{\mathbb Q}} \right| + \left| \mathbb E_{\hat{\mathbb Q}} - \mathbb E_{\mathbb Q} \right| \right] \\
        &\leq  \underset{f\in\mathcal{F}}{\text{sup}}\left| \mathbb{E}_{\hat{\mathbb P} } - \mathbb E_{\hat{\mathbb Q}} \right| + \underset{f\in\mathcal{F}}{\text{sup}} \left| \mathbb E_{\hat{\mathbb Q}} - \mathbb E_{\mathbb Q} \right|,
    \end{aligned}
\end{equation}
where $\mathbb{\hat{P}}$ denotes the empirical distribution of source tasks in the meta-training phase, $\mathbb{\hat{Q}}$ denotes the empirical distribution of the support set for target tasks in the meta-testing phase, and $\mathbb Q$ denotes the expected distribution of the query set.

For the \textit{first term} in Eq.\ref{ipm}, according to Lemma \ref{lemma_1} and Lemma \ref{lemma_2}, we can bound the result as follows:
\begin{equation}
\label{imp_first}
\begin{aligned}
    \underset{f\in\mathcal{F}}{\text{sup}}\left| \mathbb{E}_{\hat{\mathbb P} } - \mathbb E_{\hat{\mathbb Q}} \right| &\leq 2 \mathcal{R}(\mathcal{F})+\sqrt{\frac{\log(1/\epsilon)}{2m}} \\
    &\leq 2\sqrt{\frac{\nu\cdot\textrm{rank}(\Sigma_\mathrm{X})}{m}}+\sqrt{\frac{\log(1/\epsilon)}{2m}}.
\end{aligned}
\end{equation}

Similarly, for the \textit{last term} in Eq.\ref{ipm}, we can obtain the bounded result as follows:

\begin{equation}
\label{ipm_second}
\begin{aligned}
    \underset{f\in\mathcal{F}}{\text{sup}} \left| \mathbb E_{\hat{\mathbb Q}} - \mathbb E_{\mathbb Q} \right| &\leq 2 \mathcal{R}(\mathcal{F})+\sqrt{\frac{\log(1/\epsilon)}{2n_q}} \\
    &\leq 2\sqrt{\frac{\nu\cdot\textrm{rank}(\Sigma_\mathrm{X})}{n_q}}+\sqrt{\frac{\log(1/\epsilon)}{2n_q}}.
\end{aligned}
\end{equation}
Combining Eqs.\ref{imp_first} and \ref{ipm_second}, we can obtain the desired results as shown in Theorem \ref{theorem_2}. Consequently,
\begin{equation}
    \begin{aligned}
        &\underset{f\in\mathcal{F}}{\text{sup}}|\mathbb{E}_{\hat{\mathbb P} }-\mathbb E_{\mathbb Q}| \leq \underset{f\in\mathcal{F}}{\text{sup}}\left| \mathbb{E}_{\hat{\mathbb P} } - \mathbb E_{\hat{\mathbb Q}} \right| + \underset{f\in\mathcal{F}}{\text{sup}} \left| \mathbb E_{\hat{\mathbb Q}} - \mathbb E_{\mathbb Q} \right|
        \\ &\leq 2\sqrt{\frac{\nu\cdot\textrm{rank}(\Sigma_\mathrm{X})}{m}}+\sqrt{\frac{\log(1/\epsilon)}{2m}} + 2\sqrt{\frac{\nu\cdot\textrm{rank}(\sum_\mathrm{X})}{n_q}}+\sqrt{\frac{\log(1/\epsilon)}{2n_q}} \\
        &=\left(2\sqrt{\nu\cdot\text{rank}(\Sigma_{\mathrm{X}})} + \sqrt{\frac{\log(1/\epsilon)}{2}} \right) \left( \sqrt{\frac{1}{m}} + \sqrt{\frac{1}{n_q}} \right).
    \end{aligned}
\end{equation}
\end{proof}
Thus, we complete the proof. %Due to the introduction of intra-task and inter-task interpolation, $m$ increases. Furthermore, according to Lemma \ref{lemma_first}, the regularization effect can decrease $\nu$. Therefore, Theorem \ref{theorem_2} indicates that our method can reduce the generalization error of the training and test sets, thereby improving the model performance.

\section{Statistics and Descriptions of Datasets}
\label{dataset_description}
In this section, we provide detailed statistics and descriptions of the used datasets, which have been widely used in previous studies \cite{ding2020graph, liu2022few, wang2022task}. The detailed descriptions are provided below.

\noindent $\bullet$ \textbf{Amazon-Clothing} \cite{mcauley2015inferring}: It is a product network constructed from the ``Clothing, Shoes, and Jewelry'' category on Amazon. In this dataset, each product is treated as a node, and its description is used to construct node features. A link is created between products if they are co-viewed. The labels are defined as the low-level product class. For this dataset, we use the 40/17/20 class split for meta-training/meta-validation/meta-testing.

\noindent $\bullet$ \textbf{CoraFull} \cite{bojchevski2017deep}: It is a prevalent citation network. Each node represents a paper, and an edge is created between two papers if one cites the other. The nodes are labeled based on the topics of the papers. This dataset extends the previously widely used small dataset Cora by extracting raw data from the entire network. For this dataset, we use a 25/20/25 node class split for meta-training/meta-validation/meta-testing.

\noindent $\bullet$ \textbf{Amazon-Electronics} \cite{mcauley2015inferring}: It is another Amazon product network that contains products belonging to the ``Electronics" category. Each node represents a product, with its features representing the product description. An edge is created between products if there is a co-purchasing relationship. The low-level product categories are used as class labels. For this dataset, we use a 90/37/40 node category split for meta-training/meta-validation/meta-testing.

\noindent $\bullet$ \textbf{DBLP} \cite{tang2008arnetminer}: It is a citation network where each node represents a paper, and the edges represent citation relationships between different papers. The abstracts of the papers are used to construct node features. The class labels of the nodes are defined as the publication venues of the papers. For this dataset, we use an 80/27/30 node category split for meta-training/meta-validation/meta-testing.

% \begin{table}
% \renewcommand{\thetable}{S2}
% \centering
% \caption{Statistics of the datasets.}
% \label{dataset}
% \resizebox{0.45\textwidth}{!}{%
% \begin{tabular}{@{}c|ccccc@{}}
% \toprule
% Dataset            & \# Nodes & \# Edges & \# Features & \# Labels & Class Splits \\ \midrule
% Amazon-Clothing    & 24,919   & 91,680   & 9,034       & 77        & 40/17/20     \\
% CoraFull          & 19,793   & 65,311   & 8,710       & 70        & 25/20/25     \\
% Amazon-Electronics & 42,318   & 43,556   & 8,669       & 167       & 90/37/40     \\
% DBLP               & 40,672   & 288,270  & 7,202       & 137       & 80/27/30     \\ \bottomrule
% \end{tabular}%
% }
% \end{table}

\section{Descriptions of Baselines}
\label{baseline}
In this section, we present the detailed descriptions of the selected baselines below.

\subsection{Traditional Meta-learning Method}
\noindent \textbf{Protonet} \cite{snell2017prototypical}: It learns a metric space by acquiring prototypes of different categories from the support set and computes the similarity between the query samples and each prototype to predict their categories.

\noindent \textbf{MAML} \cite{finn2017model}: It enables the meta-trainer to obtain a well-initialized parameter by performing one or more gradient update steps on the model parameters, allowing for rapid adaptation to downstream novel tasks with limited labeled data.

\subsection{Meta-learning with Fewer Tasks Method}
\noindent \textbf{MetaMix} \cite{yao2021improving}: It enhances meta-training tasks by linearly combining the features and labels of samples from the support and query sets to improve the generalization of the model.

\noindent \textbf{MLTI} \cite{yao2021meta}: It generates additional tasks by randomly sampling a pair of tasks and interpolating their corresponding features and labels, replacing the original tasks for training.

\noindent \textbf{Meta-Inter} \cite{lee2022set}: It proposes a domain-agnostic task augmentation method that utilizes expressive neural set functions to densify the distribution of meta-training tasks through a bi-level optimization process.

\subsection{Graph Meta-learning Method}
\noindent \textbf{Meta-GNN} \cite{zhou2019meta}: It seamlessly integrates MAML and GNNs in a straightforward manner, leveraging the MAML framework to acquire useful prior knowledge from previous tasks during the process of learning node embeddings, enabling it to rapidly adapt to novel tasks.

\noindent \textbf{GPN} \cite{ding2020graph}: It adopts the concept of Protonet for the few-shot node classification task. It uses a GNN-based encoder and evaluator to learn node embeddings and assess the importance of these nodes, while assigning novel samples to their closest categories.

\noindent \textbf{G-Meta} \cite{huang2020graph}: It constructs an individual subgraph for each node, transmits node-specific information within these subgraphs, and employs meta-gradients to learn transferable knowledge based on the MAML framework.

\noindent \textbf{Meta-GPS} \cite{liu2022few}: It cleverly introduces prototype-based parameter initialization, scaling, and shifting transformations to better learn transferable meta-knowledge within the MAML framework and adapts to novel tasks more quickly.

%\textbf{TENT} \cite{wang2022task}: It proposes an adaptive framework comprising node-level, class-level, and task-level components, aiming to reduce the generalization gap between meta-training and meta-testing, and mitigate the impact of diverse task variations on model performance.

\noindent \textbf{X-FNC} \cite{wang2023few}: It first performs label propagation to obtain rich pseudo-labeled nodes based on Poisson learning, and then filters out irrelevant information through classifying nodes and an information bottleneck-based method to gather meta-knowledge across different meta-tasks with extremely supervised information.

\noindent \textbf{COSMIC} \cite{wang2023contrastive}: It proposes a contrastive meta-learning framework, which first explicitly aligns node embeddings by contrasting two-step optimization within each episode, and then generates hard node classes through a similarity-sensitive mixing strategy.

\noindent \textbf{TLP} \cite{tan2022transductive}: It introduces the concept of transductive linear probing, initially pretraining a graph encoder through graph contrastive learning, and then applying it to obtain node embeddings during the meta-testing phase for downstream tasks. 

\noindent \textbf{TEG} \cite{kim2023task}: It designs a task-equivariant graph few-shot learning framework, leveraging equivariant neural networks to learn adaptive task-specific strategies, aimed at capturing task inductive biases to quickly adapt to unseen tasks.

% \subsection{Graph Prompting Method}
% \textbf{GraphPrompt} \cite{liu2023graphprompt}:

% \textbf{GPF} \cite{fang2024universal}:
\subsection{Implementation Details of Baselines}
For traditional meta-learning models, we follow the same settings as \cite{ding2020graph, liu2022few}, and conduct careful hyperparameter search and report their optimal performance. For meta-learning with fewer tasks models, we uniformly use SGC as the graph encoder. Moreover, we adopt the following additional experimental settings. Specifically, for MetaMix, we allow it to perform task augmentation by generating the same number of nodes as those in the original support and query sets for each meta-training task. For MLTI and Meta-Inter, we make them to generate the same number of additional tasks as in our experiments to ensure fairness. For graph meta-learning baselines, we use the hyperparameters recommended in the original papers. All the experiments are conducted by NVIDIA 3090Ti GPUs with the Python 3.7 and PyTorch 1.13 environment.

\section{More Experimental Results}
\label{more_experiment}
\subsection{Model Performance with Sufficient Tasks}
We present the experimental results of our method and other baselines in Tables \ref{res_full} under sufficient tasks with the 5 way 5 shot setting. According to Table \ref{res_full}, we observe that the proposed SMILE achieves competitive performance compared to other baselines, thus providing strong evidence for its effectiveness in addressing the graph few-shot learning problem. %Especially when there are a few meta-training tasks, our method explicitly densify the task distribution, which can highlight its unique advantages. For instance, in the 5 tasks experimental setting on the Cora-full dataset, our method outperforms the second-best model by as much as 30\% in terms of both evaluated metrics.

Also, we provide the results of these models in more challenging cross-domain experimental settings in Table \ref{res_full_task}. In this experimental setup, we first meta-train the model on the source domain and then evaluate it on the target domain. According to the results, similar to the in-domain ones, we find that our proposed approach still significantly outperforms all baselines, %Taking the experimental setup of 5 tasks under ``Amazon-Clothing$\rightarrow$CoraFull'' as an example, SMILE leads the second-best model by more than 26\% in terms of relevant metrics. This phenomenon 
further demonstrating its ability to effectively extract transferable knowledge and exhibit strong generalization performance.

\begin{table*}[ht]
%\tiny

%\setlength{\tabcolsep}{6pt}
\centering
\caption{Results (\%) of different models with sufficient meta-training tasks under the 5-way 5-shot \textit{in-domain} setting.} %Bold: best (according to the pairwise t-test with 95\% confidence). Underline: runner-up.}
\label{res_full}
\resizebox{\textwidth}{!}{%
\begin{tabular}{@{}c|cccccccc@{}}
\toprule
\multirow{2}{*}{Model} & \multicolumn{2}{c}{Amazon-Clothing} & \multicolumn{2}{c}{CoraFull}   & \multicolumn{2}{c}{Amazon-Electronics} & \multicolumn{2}{c}{DBLP}        \\ \cmidrule(l){2-9} 
                       & Acc              & F1               & Acc            & F1             & Acc                & F1                & Acc            & F1             \\ \midrule
Protonet               & 63.51$\pm$3.62            & 63.70$\pm$2.59            & 55.65$\pm$3.76          & 52.92$\pm$3.66          & 59.72$\pm$2.69              & 61.50$\pm$2.62             & 56.32$\pm$2.39          & 55.39$\pm$2.32          \\
MAML                   & 66.12$\pm$3.12            & 67.82$\pm$2.92            & 56.52$\pm$2.70          & 55.39$\pm$3.15          & 59.02$\pm$3.49              & 58.31$\pm$3.20             & 49.93$\pm$3.62          & 47.79$\pm$3.16          \\ \midrule
MetaMix               & 83.19$\pm$2.95            & 82.12$\pm$2.56            & 70.36$\pm$2.39          & 68.59$\pm$2.69          & 78.25$\pm$3.25              & 77.09$\pm$3.11             & 80.26$\pm$2.55          & 79.06$\pm$2.59          \\
MLTI               & 83.39$\pm$2.46            & 82.56$\pm$2.30            & 70.99$\pm$2.15          & 69.39$\pm$2.56          & 79.36$\pm$2.75              & 78.12$\pm$2.56             & 81.22$\pm$2.52          & 80.16$\pm$2.36          \\
Meta-Inter                   & 85.39$\pm$2.72            & 84.26$\pm$2.19            & 73.19$\pm$2.59          & 72.65$\pm$2.35          & 80.16$\pm$2.95              & 79.49$\pm$2.76             & 81.59$\pm$2.76          & 80.96$\pm$2.52          \\ \midrule
Meta-GNN               & 74.79$\pm$2.39            & 77.50$\pm$2.52            & 59.12$\pm$2.36          & 57.12$\pm$2.56          & 67.91$\pm$3.19              & 66.83$\pm$3.32             & 74.20$\pm$2.95          & 73.10$\pm$3.19          \\
GPN                    & 76.13$\pm$2.20            & 79.03$\pm$2.39            & 60.31$\pm$2.19          & 59.46$\pm$2.36          & 70.93$\pm$2.72              & 70.64$\pm$2.79             & 76.19$\pm$2.52          & 75.82$\pm$2.35          \\
G-Meta                 & 76.62$\pm$3.25            & 78.60$\pm$3.19            & 62.43$\pm$3.11          & 61.61$\pm$2.76          & 73.62$\pm$2.52              & 72.60$\pm$3.19             & 77.61$\pm$3.26          & 76.93$\pm$3.03          \\
Meta-GPS               & 82.62$\pm$2.39            & 81.62$\pm$2.26            & 69.25$\pm$2.52          & 68.60$\pm$2.25          & 80.26$\pm$2.16        & 79.32$\pm$2.05       & 81.76$\pm$1.95          & 81.15$\pm$1.86    \\
X-FNC                  & 82.83$\pm$2.66            & 81.59$\pm$2.32            & 71.26$\pm$2.19          & 69.02$\pm$2.59          & 77.39$\pm$2.56              & 76.50$\pm$2.39             & 79.59$\pm$2.26          & 78.06$\pm$2.19          \\ 
COSMIC                   & 86.22$\pm$1.70      & 85.65$\pm$1.93      & 77.24$\pm$1.52    & 75.10$\pm$1.82    & 79.38$\pm$2.25              & 77.59$\pm$2.36             & 81.94$\pm$2.20    & 80.39$\pm$2.79          \\ 
TLP                   & 85.22$\pm$3.35      & 83.65$\pm$3.19      & 71.36$\pm$4.49    & 70.70$\pm$3.72    & 79.38$\pm$3.92              & 77.59$\pm$3.55             & 81.94$\pm$2.82    & 80.39$\pm$2.56          \\
TEG                   & \textbf{90.18$\pm$0.95}      & \textbf{89.25$\pm$1.36}      & \textbf{76.37$\pm$1.92}    & \textbf{75.76$\pm$1.25}    & \textbf{87.17$\pm$1.15}              & \textbf{85.29$\pm$2.02}             & \underline{83.33$\pm$1.22}    & \underline{82.39$\pm$1.29}          \\
\midrule
SMILE                  & \underline{88.86$\pm$1.12}   & \underline{88.59$\pm$1.16}   & \underline{75.50$\pm$1.26} & \underline{75.14$\pm$1.39} & \underline{85.55$\pm$1.62}     & \underline{84.95$\pm$1.29}    & \textbf{83.90$\pm$1.19} & \textbf{83.42$\pm$1.56} \\ \bottomrule
\end{tabular} %
}
\end{table*}

\begin{table*}[ht]
%\tiny

\centering
\caption{Results (\%) of different models with sufficient meta-training tasks under the 5-way 5-shot \textit{cross-domain} setting.}
\label{res_full_task}
\resizebox{\textwidth}{!}{ %
\begin{tabular}{@{}c|cccccccc@{}}
\toprule
\multirow{2}{*}{Dataset} & \multicolumn{2}{c}{Amazon-Clothing$\rightarrow$CoraFull} & \multicolumn{2}{c}{CoraFull$\rightarrow$Amazon-Clothing} & \multicolumn{2}{c}{Amazon-Electronics$\rightarrow$DBLP} & \multicolumn{2}{c}{DBLP$\rightarrow$Amazon-Electronics} \\ \cmidrule(l){2-9} 
                         & Acc                          & F1                          & Acc                          & F1                          & Acc                         & F1                          & Acc                         & F1                          \\ \midrule
Protonet                 & 36.46$\pm$3.19                        & 22.85$\pm$2.72                       & 36.52$\pm$2.93                        & 33.36$\pm$2.90                       & 42.76$\pm$2.78                       & 39.30$\pm$2.72                       & 37.86$\pm$2.66                       & 29.47$\pm$2.62                       \\
MAML                     & 34.01$\pm$3.39                        & 20.95$\pm$3.12                       & 35.19$\pm$2.96                        & 34.29$\pm$2.60                       & 38.47$\pm$3.10                       & 32.51$\pm$3.19                       & 35.92$\pm$2.70                       & 26.70$\pm$3.06                       \\ \midrule
MetaMix               & 40.16$\pm$2.13            & 38.25$\pm$2.39            & 44.19$\pm$2.56          & 42.39$\pm$2.92          & 53.10$\pm$2.42              & 51.90$\pm$2.35             & 47.36$\pm$2.56          & 45.19$\pm$2.32          \\
MLTI               & 43.35$\pm$2.11            & 42.10$\pm$2.09            &  48.20$\pm$2.33         & 46.26$\pm$2.17          & 55.11$\pm$2.77              & 53.49$\pm$2.60             & 49.10$\pm$2.09          & 47.06$\pm$2.46          \\
Meta-Inter                   & 45.36$\pm$2.39            & 43.25$\pm$2.11            & 49.15$\pm$2.66          & 47.36$\pm$2.72          & 56.39$\pm$2.40              & 55.16$\pm$2.30             & 49.39$\pm$2.59          & 47.49$\pm$2.56          \\ \midrule
Meta-GNN                 & 37.29$\pm$2.56                        & 31.66$\pm$2.49                       & 45.79$\pm$2.32                        & 43.72$\pm$2.29                       & 50.16$\pm$2.30                       & 49.76$\pm$2.36                       & 45.66$\pm$2.29                       & 43.66$\pm$2.25                       \\
GPN                      & 45.26$\pm$3.35                  & 43.25$\pm$3.12                 & 56.16$\pm$2.99                        & 55.68$\pm$2.75                       & \underline{65.28$\pm$2.42}                 &\underline{65.37$\pm$2.53}                 & 49.20$\pm$3.39                       & 47.62$\pm$3.40                       \\
G-Meta                   & 39.39$\pm$3.41                        & 38.72$\pm$2.95                       & 49.90$\pm$2.75                        & 48.56$\pm$2.96                       & 55.26$\pm$2.47                       & 53.75$\pm$2.49                       & 46.72$\pm$2.32                       & 45.67$\pm$2.29                       \\
Meta-GPS                 & 41.29$\pm$2.16                        & 40.79$\pm$2.12                       & \underline{58.62$\pm$2.25}                        & \underline{57.29$\pm$2.20}                       & 60.12$\pm$2.06                       & 59.73$\pm$2.02                       & 49.39$\pm$2.15                       & \underline{47.96$\pm$2.12}                       \\
%TENT                     & 43.09                        & 42.72                       & \underline{58.92}                  & \underline{57.79}                 & 62.17                       & 61.56                       & \underline{50.29}                 & \underline{49.73}                 \\
X-FNC                    & 42.56$\pm$2.75                        & 41.19$\pm$2.46                       & 55.39$\pm$2.49                        & 54.29$\pm$2.37                       & 61.55$\pm$2.32                       & 60.92$\pm$2.74                       & 49.21$\pm$2.51                       & 46.55$\pm$2.39                       \\ 
COSMIC                    & \underline{46.55$\pm$2.45}                        & \underline{44.29$\pm$2.42}                       & 57.26$\pm$2.39                        & 56.22$\pm$2.40                       & 63.59$\pm$2.98                       & 62.29$\pm$2.93                       & 51.22$\pm$2.86                       & 50.35$\pm$2.78                       \\
TLP                    & 44.76$\pm$3.47                        & 43.29$\pm$3.32                       & 57.95$\pm$2.91                        & 56.36$\pm$2.77                       & 64.52$\pm$2.73                       & 63.22$\pm$2.49                       & \underline{49.51$\pm$2.36}                       & 46.55$\pm$2.72                       \\
TEG                    & 40.19$\pm$1.26                        & 39.96$\pm$1.66                       & 50.23$\pm$2.53                        & 48.29$\pm$2.06                       & 46.35$\pm$2.65                       & 45.26$\pm$2.72                       & 41.25$\pm$1.93                       & 40.59$\pm$1.60                       \\ \midrule
SMILE                    & \textbf{49.08$\pm$1.23}               & \textbf{47.46$\pm$1.42}              & \textbf{62.72$\pm$2.02}               & \textbf{61.29$\pm$1.86}              & \textbf{68.96$\pm$1.12}              & \textbf{68.03$\pm$1.06}              & \textbf{53.38$\pm$1.32}              & \textbf{52.70$\pm$1.25}              \\ \bottomrule
\end{tabular} %
}
\end{table*}

\subsection{Comparison of Performance with With-in Task Mixup and Increased Shot Numbers}

\begin{table*}[ht]
%\tiny
\scriptsize

\centering
\caption{Results of our model on the 5-way 5-shot 5 tasks in-domain setting compared with those of other models on the 5-way 10-shot 5 tasks setting.}
\label{res_many_shot}
\resizebox{\textwidth}{!}{%
\begin{tabular}{@{}c|cccccccc@{}}
\toprule
\multirow{2}{*}{Model} & \multicolumn{2}{c}{Amazon-Clothing} & \multicolumn{2}{c}{CoraFull}    & \multicolumn{2}{c}{Amazon-Electronics} & \multicolumn{2}{c}{DBLP}        \\ \cmidrule(l){2-9} 
                       & Acc               & F1               & Acc            & F1             & Acc                & F1                & Acc            & F1             \\ \midrule
Protonet               & 49.27$\pm$3.19             & 48.72$\pm$2.79            & 38.95$\pm$2.61          & 37.87$\pm$2.68          & 50.14$\pm$2.73              & 49.80$\pm$2.65             & 50.91$\pm$2.56          & 49.99$\pm$2.73          \\
MAML                   & 46.42$\pm$2.30             & 45.16$\pm$2.34            & 40.12$\pm$2.35          & 38.79$\pm$2.56          & 39.95$\pm$2.62              & 38.60$\pm$2.71             & 45.26$\pm$2.42          & 43.92$\pm$2.93          \\ \midrule
% MetaMix               &             &             &           &           &               &              &           &           \\
% MLTI               &             &             &           &           &               &              &           &           \\
% Meta-Inter                   &             &             &           &           &               &              &           &           \\ \midrule
Meta-GNN               & 57.06$\pm$3.72             & 53.19$\pm$3.47            & 43.90$\pm$3.12          & 42.19$\pm$3.09          & 45.16$\pm$2.19              & 43.96$\pm$2.15             & 52.35$\pm$2.35          & 51.76$\pm$2.32          \\
GPN                    & 68.64$\pm$2.73             & 68.39$\pm$2.07            & 45.22$\pm$3.45          & 43.29$\pm$3.21          & 54.23$\pm$2.73              & 53.17$\pm$2.50             & 70.39$\pm$2.29          & 70.13$\pm$2.65          \\
G-Meta                 & 61.29$\pm$2.59             & 60.96$\pm$2.32            & 46.72$\pm$2.40          & 45.35$\pm$2.49          & 45.20$\pm$3.12              & 43.56$\pm$3.22             & 53.99$\pm$2.93          & 49.20$\pm$2.71          \\
Meta-GPS               & 63.22$\pm$2.35             & 60.36$\pm$2.29            & 52.16$\pm$2.19          & 50.10$\pm$2.11          & 49.32$\pm$2.95              & 46.02$\pm$2.62             & 58.19$\pm$1.98          & 56.22$\pm$1.72          \\
X-FNC                  & 70.22$\pm$2.97       & 69.35$\pm$2.73            & 56.99$\pm$2.65          & 53.96$\pm$2.42          & 62.19$\pm$2.34              & 59.39$\pm$2.47             & 71.66$\pm$2.39          & 70.92$\pm$2.91          \\ 
COSMIC                   & 77.29$\pm$2.93             & 76.33$\pm$2.82      & \underline{64.22$\pm$2.53}    & 62.33$\pm$2.45    & 65.25$\pm$2.46        & 64.18$\pm$2.72 & 72.10$\pm$3.16    & 71.15$\pm$3.06    \\ 
TLP                   & 73.21$\pm$2.29             & 72.13$\pm$2.12      & 53.11$\pm$2.35    & 52.01$\pm$2.19    & 64.51$\pm$2.77        & 63.18$\pm$3.02       & 72.39$\pm$3.03    & 71.35$\pm$3.12    \\
TEG                   & \underline{80.22$\pm$2.12}             & \underline{79.36$\pm$2.36}      & 64.16$\pm$1.76    & \underline{63.31$\pm$1.63}    & \underline{66.06$\pm$1.96}        & \underline{65.16$\pm$1.95}       & \underline{74.36$\pm$2.03}    & \underline{73.19$\pm$2.39}    \\ \midrule
SMILE                  & \textbf{82.80$\pm$1.32}    & \textbf{82.49$\pm$1.52}   & \textbf{66.34$\pm$1.29} & \textbf{65.70$\pm$1.56} & \textbf{67.30$\pm$1.20}     & \textbf{66.30$\pm$1.19}    & \textbf{75.88$\pm$1.29} & \textbf{75.05$\pm$1.36} \\ \bottomrule
\end{tabular}%
}
\end{table*}

Further, %We conduct an interesting experiment to compare our model against baselines with explicitly increased shots using external data. Since we perform intra-task mixup that doubles the original shot number, we would like to examine how our model performs relative to baselines, despite our augmented data coming from within task distributions. Specifically, we adopt the 5-way 5-shot setting with 5 tasks, and generate doubled shot in each task by default. Thus, for the baselines, we adopt the 5-way 10-shot setting with external data sampling.
%we also conduct an interesting experiment to investigate the performance of our model with intra-task mixup compared to baselines that increase the number of shots with external data. Since we explicitly perform intra-task mixup, we wanted to examine how our model performs relative to baselines with explicitly increased shots from external sources, despite our augmented data coming from within task distributions. 
we conduct an interesting experiment to explore how our model augmented via within-task mixup fares against baselines enhanced by increasing shot count with external data. While our augmented data originates from within task distributions, we aim to evaluate its effectiveness compared to baselines explicitly inflated with external data. Specifically, we ran experiments using the 5-way 5-shot setting with five tasks on all datasets. As within-task mixup effectively doubles the shot count, we opt for the 5-way 10-shot setting for the baselines. %Specifically, we conduct the experiments under the 5-way 5-shot with five tasks. Since intra-task mixup is equivalent to doubling the number of shots, we choose the 5-way 10-shot setting for the baselines. 
Note that we have not included meta-learning with fewer tasks methods (\textit{i.e.}, MetaMix, MLTI, and Meta-Inter) here, as they have already explicitly performed data augmentation or task augmentation. According to Table \ref{res_many_shot}, we find that baseline models exhibit slight performance improvements from 5-way 5-shot to 5-way 10-shot settings, yet they still fail to outperform our model. This further highlights the superiority of SMILE. %baseline models show slight improvements in performance from 5-way 5-shot to 5-way 10-shot, but still do not outperform our model, further demonstrating the superiority of SMILE.

\subsection{Model Performance with Alternative Across-task Mixup}
\label{alternative_mixup}
To further demonstrate the superiority of our proposed across-task mixup, we attempt to replace it with the mixup strategy in the MLTI \cite{yao2021meta}. It directly performs mixup on the support set and query set from two tasks to achieve task augmentation, formally defined as:
\begin{equation}
    \begin{aligned}
        \tilde{\mathrm{X}}_{t;\tilde{k}}^s\!=\!\lambda\mathrm{X}_{i;k}^s\!+\!(1\!-\!\lambda)\mathrm{X}_{j;k^\prime}^s, \quad
        \tilde{\mathrm{X}}_{t;\tilde{k}}^q\!=\!\lambda\mathrm{X}_{i;k}^q\!+\!(1\!-\!\lambda)\mathrm{X}_{j;k^\prime}^q.
    \end{aligned}
\end{equation}
We present the results with different mixup strategies under the 5-way 5-shot in-domain and cross-domain settings varying number of tasks in Table \ref{mixup_res}. Here, ``\textit{alternate}'' denotes the model variant that  performs the aforementioned task augmentation.

\begin{table*}[ht]

\caption{Results (\%) of different model variants on the datasets under various experimental settings.}
\label{mixup_res}
\resizebox{\textwidth}{!}{%
\begin{tabular}{@{}c|c|cccccccc@{}}
\toprule
\multirow{2}{*}{Task} & \multirow{2}{*}{Model} & \multicolumn{2}{c}{Amazon-Clothing}                        & \multicolumn{2}{c}{CoraFull}                               & \multicolumn{2}{c}{Amazon-Electronics}                    & \multicolumn{2}{c}{DBLP}                                  \\ \cmidrule(l){3-10} 
                      &                        & Acc                          & F1                          & Acc                          & F1                          & Acc                         & F1                          & Acc                         & F1                          \\ \midrule
\multirow{2}{*}{5}    & \textit{alternate}                 & 81.69$\pm$1.39                   & 81.52$\pm$1.22                  & 65.42$\pm$1.70                   & 64.79$\pm$1.35                  & 65.96$\pm$1.19                  & 65.20$\pm$1.22                  & 74.92$\pm$1.32                  & 73.95$\pm$1.15                  \\
                      & ours                   & \textbf{82.80$\pm$1.32}          & \textbf{82.49$\pm$1.52}         & \textbf{66.34$\pm$1.29}          & \textbf{65.70$\pm$1.56}         & \textbf{67.30$\pm$1.20}         & \textbf{66.30$\pm$1.19}         & \textbf{75.88$\pm$1.29}         & \textbf{75.05$\pm$1.36}         \\ \midrule
\multirow{2}{*}{10}   & \textit{alternate}                 & 82.22$\pm$1.50                   & 82.02$\pm$1.12                  & 70.79$\pm$1.26                   & 70.22$\pm$1.32                  & 69.99$\pm$1.02                  & 69.16$\pm$1.39                  & 75.26$\pm$1.70                  & 73.90$\pm$1.96                  \\
                      & ours                   & \textbf{83.46$\pm$1.66}          & \textbf{82.88$\pm$1.35}         & \textbf{71.72$\pm$1.95}          & \textbf{71.15$\pm$1.76}         & \textbf{70.76$\pm$1.06}         & \textbf{70.05$\pm$1.09}         & \textbf{76.64$\pm$1.22}         & \textbf{75.77$\pm$1.19}         \\ \midrule
\multirow{2}{*}{15}   & \textit{alternate}                 & 82.99$\pm$1.29                   & 82.39$\pm$1.36                  & 69.72$\pm$1.52                   & 69.03$\pm$1.32                  & 72.25$\pm$1.39                  & 71.12$\pm$1.47                  & 78.52$\pm$1.56                  & 77.35$\pm$1.30                  \\
                      & ours                   & \textbf{83.92$\pm$1.16}          & \textbf{83.33$\pm$1.22}         & \textbf{70.78$\pm$1.59}          & \textbf{70.19$\pm$1.42}         & \textbf{73.48$\pm$1.36}         & \textbf{72.66$\pm$1.22}         & \textbf{79.56$\pm$1.26}         & \textbf{78.77$\pm$1.76}         \\ \midrule
\multirow{2}{*}{20}   & \textit{alternate}                 & 83.72$\pm$1.38                   & 82.95$\pm$1.49                  & 71.92$\pm$1.71                   & 71.72$\pm$1.96                  & 74.39$\pm$1.86                  & 74.32$\pm$1.72                  & 79.52$\pm$1.39                  & 78.51$\pm$1.77                  \\
                      & ours                   & \textbf{84.66$\pm$1.55}          & \textbf{84.52$\pm$1.39}         & \textbf{72.60$\pm$1.66}          & \textbf{72.10$\pm$1.55}         & \textbf{75.42$\pm$1.52}         & \textbf{75.42$\pm$1.29}         & \textbf{80.50$\pm$1.72}         & \textbf{79.61$\pm$1.55}         \\ \midrule
\multirow{2}{*}{Task} & \multirow{2}{*}{Model} & \multicolumn{2}{c}{Amazon-Clothing$\rightarrow$CoraFull} & \multicolumn{2}{c}{CoraFull$\rightarrow$Amazon-Clothing} & \multicolumn{2}{c}{Amazon-Electronics$\rightarrow$DBLP} & \multicolumn{2}{c}{DBLP$\rightarrow$Amazon-Electronics} \\ \cmidrule(l){3-10} 
                      &                        & Acc                          & F1                          & Acc                          & F1                          & Acc                         & F1                          & Acc                         & F1                          \\ \midrule
\multirow{2}{*}{5}    & \textit{alternate}                 & 42.02$\pm$2.36                   & 41.42$\pm$1.72                  & 55.37$\pm$1.97                   & 54.36$\pm$1.86                  & 61.30$\pm$1.79                  & 61.02$\pm$1.75                  & 45.14$\pm$1.39                  & 43.72$\pm$1.55                  \\
                      & ours                   & \textbf{42.64$\pm$2.02}          & \textbf{41.27$\pm$1.65}         & \textbf{56.36$\pm$2.02}          & \textbf{55.25$\pm$1.75}         & \textbf{62.44$\pm$1.35}         & \textbf{61.66$\pm$1.29}         & \textbf{46.24$\pm$1.60}         & \textbf{44.54$\pm$1.62}         \\ \midrule
\multirow{2}{*}{10}   & \textit{alternate}                 & 43.59$\pm$1.22                   & 41.79$\pm$1.59                  & 57.99$\pm$1.73                   & 56.76$\pm$1.62                  & 63.12$\pm$1.79                  & 62.29$\pm$2.25                  & 47.95$\pm$2.22                  & 46.82$\pm$2.16                  \\
                      & ours                   & \textbf{45.14$\pm$1.29}          & \textbf{43.69$\pm$1.10}         & \textbf{58.84$\pm$1.79}          & \textbf{57.53$\pm$1.56}         & \textbf{64.54$\pm$1.22}         & \textbf{64.16$\pm$1.20}         & \textbf{48.82$\pm$1.12}         & \textbf{47.26$\pm$1.19}         \\ \midrule
\multirow{2}{*}{15}   & \textit{alternate}                 & 45.12$\pm$1.77                   & 43.39$\pm$1.56                  & 58.16$\pm$1.32                   & 54.76$\pm$1.39                  & 63.70$\pm$1.42                  & 63.26$\pm$1.49                  & 48.39$\pm$1.51                  & 46.89$\pm$1.60                  \\
                      & ours                   & \textbf{45.88$\pm$1.36}          & \textbf{44.10$\pm$1.22}         & \textbf{59.08$\pm$1.55}          & \textbf{55.96$\pm$1.50}         & \textbf{65.04$\pm$1.19}         & \textbf{64.43$\pm$1.26}         & \textbf{49.26$\pm$1.55}         & \textbf{47.70$\pm$1.36}         \\ \midrule
\multirow{2}{*}{20}   & \textit{alternate}                 & 46.12$\pm$1.09                   & 44.26$\pm$1.75                  & 57.99$\pm$1.79                   & 57.56$\pm$1.73                  & 63.92$\pm$1.60                  & 63.22$\pm$1.92                  & 47.28$\pm$1.50                  & 47.06$\pm$1.35                  \\
                      & ours                   & \textbf{46.72$\pm$1.96}          & \textbf{45.65$\pm$1.66}         & \textbf{59.38$\pm$1.62}          & \textbf{58.25$\pm$1.60}         & \textbf{65.78$\pm$1.32}         & \textbf{65.42$\pm$1.26}         & \textbf{49.52$\pm$1.29}         & \textbf{47.88$\pm$1.26}         \\ \bottomrule
\end{tabular}%
}
\end{table*}

According to the results, we can conclude that the adopted across-task augmentation strategy consistently outperforms the task augmentation of MLTI on various experimental settings. One plausible reason is that the adopted prototype-based across-task mixup can generate more reliable data compared to instance-based one of other models, thus further reducing adverse oscillations when predicting examples beyond the training set. %under the constraints of prototypes, the data generated through mixup has better controllability.

\subsection{Impact of Original Tasks}
\label{ori_task}
%In our designed model, during the meta-training stage, we explicitly utilize the original tasks $\mathcal{D}_{org}$, whereas MLTI disregards the use of them and only is trained on the generated new tasks $\mathcal{D}_{aug}$. 
Our proposed model is trained during the meta-training stage utilizing a merged task $\mathcal{D}_{all}$ composed of original tasks $\mathcal{D}_{org}$ and interpolated tasks $\mathcal{D}_{aug}$. In contrast, MLTI disregards the use of original tasks and solely uses the generated new tasks for training. However, this approach raises concerns as the model does not directly encounter the data distribution of the original tasks, potentially compromising its generalization ability. Moreover, in scenarios where training data is already scarce, this practice results in the wastage of valuable data resources. To further quantitatively explore the impact of these original tasks on model performance, we conduct additional experiments with several model variants under different experimental settings across all the datasets. Here, ``\textit{w/o original taks}'' denotes that we exclude the original tasks and solely rely on the generated tasks for model training. All the results are presented in Table \ref{wo_ori_res}.

\begin{table*}[ht]

\caption{Results (\%) of different training methods on the datasets.}
\label{wo_ori_res}
\resizebox{\textwidth}{!}{%
\begin{tabular}{@{}c|c|cccccccc@{}}
\toprule
\multirow{2}{*}{Task} & \multirow{2}{*}{Model} & \multicolumn{2}{c}{Amazon-Clothing}                        & \multicolumn{2}{c}{CoraFull}                               & \multicolumn{2}{c}{Amazon-Electronics}                    & \multicolumn{2}{c}{DBLP}                                  \\ \cmidrule(l){3-10} 
                      &                        & Acc                          & F1                          & Acc                          & F1                          & Acc                         & F1                          & Acc                         & F1                          \\ \midrule
\multirow{2}{*}{5}    & \textit{w/o original tasks}                & 81.74$\pm$1.79                   & 81.60$\pm$1.69                  & 65.69$\pm$1.75                   & 64.72$\pm$1.52                  & 65.36$\pm$1.22                  & 64.20$\pm$1.29                  & 74.05$\pm$1.36                  & 73.09$\pm$1.19                  \\
                      & ours                   & \textbf{82.80$\pm$1.32}          & \textbf{82.49$\pm$1.52}         & \textbf{66.34$\pm$1.29}          & \textbf{65.70$\pm$1.56}         & \textbf{67.30$\pm$1.20}         & \textbf{66.30$\pm$1.19}         & \textbf{75.88$\pm$1.29}         & \textbf{75.05$\pm$1.36}         \\ \midrule
\multirow{2}{*}{10}   & \textit{w/o original tasks}                 & 82.06$\pm$1.55                   & 81.36$\pm$1.19                  & 70.29$\pm$1.32                   & 69.95$\pm$1.36                  & 69.09$\pm$1.42                  & 68.16$\pm$1.33                  & 75.36$\pm$1.75                  & 72.90$\pm$1.73                  \\
                      & ours                   & \textbf{83.46$\pm$1.66}          & \textbf{82.88$\pm$1.35}         & \textbf{71.72$\pm$1.95}          & \textbf{71.15$\pm$1.76}         & \textbf{70.76$\pm$1.06}         & \textbf{70.05$\pm$1.09}         & \textbf{76.64$\pm$1.22}         & \textbf{75.77$\pm$1.19}         \\ \midrule
\multirow{2}{*}{15}   & \textit{w/o original tasks}                 & 82.93$\pm$1.32                   & 81.99$\pm$1.56                  & 69.92$\pm$1.31                   & 68.26$\pm$1.37                  & 72.29$\pm$1.19                  & 71.20$\pm$1.40                  & 78.39$\pm$1.52                  & 77.20$\pm$1.35                  \\ 
                      & ours                   & \textbf{83.92$\pm$1.16}          & \textbf{83.33$\pm$1.22}         & \textbf{70.78$\pm$1.59}          & \textbf{70.19$\pm$1.42}         & \textbf{73.48$\pm$1.36}         & \textbf{72.66$\pm$1.22}         & \textbf{79.56$\pm$1.26}         & \textbf{78.77$\pm$1.76}         \\ \midrule
\multirow{2}{*}{20}   & \textit{w/o original tasks}                 & 83.69$\pm$1.39                   & 83.26$\pm$1.42                  & 71.90$\pm$1.52                   & 70.72$\pm$1.94                  & 74.29$\pm$1.26                  & 73.29$\pm$1.71                  & 79.49$\pm$1.93                  & 78.39$\pm$1.78                  \\
                      & ours                   & \textbf{84.66$\pm$1.55}          & \textbf{84.52$\pm$1.39}         & \textbf{72.60$\pm$1.66}          & \textbf{72.10$\pm$1.55}         & \textbf{75.42$\pm$1.52}         & \textbf{75.42$\pm$1.29}         & \textbf{80.50$\pm$1.72}         & \textbf{79.61$\pm$1.55}         \\ \midrule
\multirow{2}{*}{Task} & \multirow{2}{*}{Model} & \multicolumn{2}{c}{Amazon-Clothing$\rightarrow$CoraFull} & \multicolumn{2}{c}{CoraFull$\rightarrow$Amazon-Clothing} & \multicolumn{2}{c}{Amazon-Electronics$\rightarrow$DBLP} & \multicolumn{2}{c}{DBLP$\rightarrow$Amazon-Electronics} \\ \cmidrule(l){3-10} 
                      &                        & Acc                          & F1                          & Acc                          & F1                          & Acc                         & F1                          & Acc                         & F1                          \\ \midrule
\multirow{2}{*}{5}    & \textit{w/o original tasks}                 & 41.32$\pm$2.09                   & 40.56$\pm$1.71                  & 55.29$\pm$1.67                   & 53.76$\pm$1.66                  & 61.26$\pm$1.73                  & 60.10$\pm$1.69                  & 45.15$\pm$1.32                  & 43.69$\pm$1.59                  \\
                      & ours                   & \textbf{42.64$\pm$2.02}          & \textbf{41.27$\pm$1.65}         & \textbf{56.36$\pm$2.02}          & \textbf{55.25$\pm$1.75}         & \textbf{62.44$\pm$1.35}         & \textbf{61.66$\pm$1.29}         & \textbf{46.24$\pm$1.60}         & \textbf{44.54$\pm$1.62}         \\ \midrule
\multirow{2}{*}{10}   & \textit{w/o original tasks}                 & 43.56$\pm$1.29                   & 41.66$\pm$1.53                  & 57.29$\pm$1.66                   & 56.65$\pm$1.60                  & 63.09$\pm$1.39                  & 62.16$\pm$2.12                  & 47.32$\pm$2.23                  & 46.92$\pm$2.11                  \\
                      & ours                   & \textbf{45.14$\pm$1.29}          & \textbf{43.69$\pm$1.10}         & \textbf{58.84$\pm$1.79}          & \textbf{57.53$\pm$1.56}         & \textbf{64.54$\pm$1.22}         & \textbf{64.16$\pm$1.20}         & \textbf{48.82$\pm$1.12}         & \textbf{47.26$\pm$1.19}         \\ \midrule
\multirow{2}{*}{15}   & \textit{w/o original tasks}                 & 44.23$\pm$1.27                   & 43.92$\pm$1.67                  & 57.90$\pm$1.34                   & 55.29$\pm$1.31                  & 64.29$\pm$1.44                  & 63.20$\pm$1.40                  & 48.29$\pm$1.39                  & 46.29$\pm$1.63                  \\
                      & ours                   & \textbf{45.88$\pm$1.36}          & \textbf{44.10$\pm$1.22}         & \textbf{59.08$\pm$1.55}          & \textbf{55.96$\pm$1.50}         & \textbf{65.04$\pm$1.19}         & \textbf{64.43$\pm$1.26}         & \textbf{49.26$\pm$1.55}         & \textbf{47.70$\pm$1.36}         \\ \midrule
\multirow{2}{*}{20}   & \textit{w/o original tasks}                 & 45.66$\pm$1.11                   & 43.69$\pm$1.72                  & 57.97$\pm$1.73                   & 57.22$\pm$1.60                  & 64.26$\pm$1.35                  & 63.22$\pm$1.46                  & 48.46$\pm$1.59                  & 46.29$\pm$1.23                  \\
                      & ours                   & \textbf{46.72$\pm$1.96}          & \textbf{45.65$\pm$1.66}         & \textbf{59.38$\pm$1.62}          & \textbf{58.25$\pm$1.60}         & \textbf{65.78$\pm$1.32}         & \textbf{65.42$\pm$1.26}         & \textbf{49.52$\pm$1.29}         & \textbf{47.88$\pm$1.26}         \\ \bottomrule
\end{tabular}%
}
\end{table*}
Based on the above results, the training strategy utilized consistently brings about performance improvements compared to solely training the model on generated new tasks. This further underscore the effectiveness of our employed training method.

\subsection{Impact of Graph Augmentation}
In this work, we actually employ feature-level mixup. We would like to explain our rationale. Firstly, mixup is a simple and highly effective technique that aligns with the straightforward concept we aim to convey in our research. Secondly, by employing feature-level mixup, we can directly address the scarcity of nodes and tasks within a given task by enriching both the node and task distributions. Given that the target data is graph-structured data, someone may wonder how the model performance would be affected by utilizing other augmentation methods designed for graph-structured data instead of mixup. We argue that using graph augmentation methods would primarily impact the learning of node representations and would have minimal influence on subsequent algorithms that extract generalizable knowledge from limited data. To verify our hypothesis, we utilize GAug \cite{zhao2021data} and GMix \cite{wang2021mixup} for graph augmentation on the vanilla SGC \cite{wu2019simplifying} node representation learning module. Subsequently, we directly conduct metric-based few-shot node classification without introduced dual-level mixup techniques. The corresponding model variants are denoted as ``w GAug'' and ``w GMix''. Moreover, ``SGC'' denotes that we directly utilize SGC for node representation learning and subsequently perform metric-based few-shot node classification. The experimental results are presented in Table \ref{wo_graph_aug}.

\begin{table*}[ht]

\caption{Results (\%) of different models on the datasets.}
\label{wo_graph_aug}
\resizebox{\textwidth}{!}{%
\begin{tabular}{@{}c|c|cccccccc@{}}
\toprule
\multirow{2}{*}{Task} & \multirow{2}{*}{Model} & \multicolumn{2}{c}{Amazon-Clothing}                        & \multicolumn{2}{c}{CoraFull}                               & \multicolumn{2}{c}{Amazon-Electronics}                    & \multicolumn{2}{c}{DBLP}                                  \\ \cmidrule(l){3-10} 
                      &                        & Acc                          & F1                          & Acc                          & F1                          & Acc                         & F1                          & Acc                         & F1                          \\ \midrule
\multirow{4}{*}{5}    & SGC                    & 69.02$\pm$1.94                   & 67.12$\pm$1.65                  & 43.02$\pm$1.75                   & 42.29$\pm$1.50                  & 50.20$\pm$1.26                  & 47.92$\pm$1.23                  & 70.11$\pm$1.33                  & 69.25$\pm$1.15                  \\
                      & w GAug                 & 69.22$\pm$1.29                   & 67.55$\pm$1.35                  & 43.56$\pm$2.29                   & 42.39$\pm$2.17                  & 50.26$\pm$1.74                  & 47.99$\pm$1.70                  & 70.39$\pm$1.59                  & 69.39$\pm$1.24                  \\
                      & w GMix                 & 70.26$\pm$1.51                   & 68.36$\pm$1.26                  & 45.29$\pm$1.17                   & 44.02$\pm$1.39                  & 51.92$\pm$1.56                  & 49.39$\pm$1.39                  & 71.30$\pm$1.32                  & 70.70$\pm$1.20                  \\
                      & ours                   & \textbf{82.80$\pm$1.32}          & \textbf{82.49$\pm$1.52}         & \textbf{66.34$\pm$1.29}          & \textbf{65.70$\pm$1.56}         & \textbf{67.30$\pm$1.20}         & \textbf{66.30$\pm$1.19}         & \textbf{75.88$\pm$1.29}         & \textbf{75.05$\pm$1.36}         \\ \midrule
\multirow{4}{*}{10}   & SGC                    & 71.29$\pm$2.25                   & 70.32$\pm$2.19                  & 46.11$\pm$1.73                   & 44.72$\pm$1.95                  & 52.10$\pm$2.13                  & 53.56$\pm$2.36                  & 74.39$\pm$1.94                  & 73.52$\pm$1.75                  \\
                      & w GAug                 & 71.66$\pm$2.02                   & 70.62$\pm$2.13                  & 46.29$\pm$1.97                   & 44.99$\pm$1.92                  & 52.19$\pm$2.12                  & 53.66$\pm$2.49                  & 74.56$\pm$2.03                  & 73.92$\pm$1.59                  \\
                      & w GMix                 & 72.90$\pm$1.90                   & 71.36$\pm$1.75                  & 48.09$\pm$2.05                   & 45.92$\pm$2.13                  & 53.59$\pm$2.06                  & 54.02$\pm$2.31                  & 75.30$\pm$2.19                  & 74.12$\pm$2.37                  \\
                      & ours                   & \textbf{83.46$\pm$1.66}          & \textbf{82.88$\pm$1.35}         & \textbf{71.72$\pm$1.95}          & \textbf{71.15$\pm$1.76}         & \textbf{70.76$\pm$1.06}         & \textbf{70.05$\pm$1.09}         & \textbf{76.64$\pm$1.22}         & \textbf{75.77$\pm$1.19}         \\ \midrule
\multirow{4}{*}{15}   & SGC                    & 72.12$\pm$1.62                   & 71.49$\pm$1.51                  & 51.96$\pm$1.36                   & 50.20$\pm$1.35                  & 55.02$\pm$1.39                  & 54.12$\pm$1.47                  & 76.22$\pm$1.57                  & 75.12$\pm$1.65                  \\
                      & w GAug                 & 72.53$\pm$1.79                   & 71.99$\pm$2.05                  & 52.06$\pm$1.49                   & 50.36$\pm$1.70                  & 55.29$\pm$1.96                  & 54.20$\pm$1.71                  & 76.59$\pm$2.13                  & 75.26$\pm$2.03                  \\
                      & w GMix                 & 73.56$\pm$1.72                   & 72.26$\pm$1.59                  & 54.29$\pm$1.77                   & 51.20$\pm$1.67                  & 56.49$\pm$1.72                  & 55.39$\pm$1.40                  & 77.29$\pm$1.93                  & 76.12$\pm$2.14                  \\
                      & ours                   & \textbf{83.92$\pm$1.16}          & \textbf{83.33$\pm$1.22}         & \textbf{70.78$\pm$1.59}          & \textbf{70.19$\pm$1.42}         & \textbf{73.48$\pm$1.36}         & \textbf{72.66$\pm$1.22}         & \textbf{79.56$\pm$1.26}         & \textbf{78.77$\pm$1.76}         \\ \midrule
\multirow{4}{*}{20}   & SGC                    & 72.66$\pm$1.79                   & 72.16$\pm$1.49                  & 56.35$\pm$1.57                   & 55.32$\pm$1.92                  & 57.52$\pm$1.56                  & 56.69$\pm$1.75                  & 76.99$\pm$1.91                  & 76.52$\pm$1.72                  \\
                      & w GAug                 & 73.06$\pm$2.02                   & 72.36$\pm$1.99                  & 56.25$\pm$1.97                   & 55.29$\pm$1.72                  & 57.36$\pm$1.96                  & 56.49$\pm$1.47                  & 76.90$\pm$2.20                  & 76.02$\pm$2.14                  \\
                      & w GMix                 & 73.66$\pm$1.95                   & 72.99$\pm$1.73                  & 57.29$\pm$1.60                   & 56.92$\pm$1.95                  & 59.90$\pm$2.09                  & 58.20$\pm$2.03                  & 77.32$\pm$1.76                  & 77.20$\pm$1.65                  \\
                      & ours                   & \textbf{84.66$\pm$1.55}          & \textbf{84.52$\pm$1.39}         & \textbf{72.60$\pm$1.66}          & \textbf{72.10$\pm$1.55}         & \textbf{75.42$\pm$1.52}         & \textbf{75.42$\pm$1.29}         & \textbf{80.50$\pm$1.72}         & \textbf{79.61$\pm$1.55}         \\ \midrule
\multirow{2}{*}{Task} & \multirow{2}{*}{Model} & \multicolumn{2}{c}{Amazon-Clothing$\rightarrow$CoraFull} & \multicolumn{2}{c}{CoraFull$\rightarrow$Amazon-Clothing} & \multicolumn{2}{c}{Amazon-Electronics$\rightarrow$DBLP} & \multicolumn{2}{c}{DBLP$\rightarrow$Amazon-Electronics} \\ \cmidrule(l){3-10} 
                      &                        & Acc                          & F1                          & Acc                          & F1                          & Acc                         & F1                          & Acc                         & F1                          \\ \midrule
\multirow{4}{*}{5}    & SGC                    & 36.22$\pm$2.03                   & 35.15$\pm$1.75                  & 41.06$\pm$1.62                   & 40.13$\pm$1.60                  & 59.99$\pm$1.72                  & 58.91$\pm$1.63                  & 43.02$\pm$1.71                  & 43.02$\pm$1.54                  \\
                      & w GAug                 & 36.42$\pm$2.17                   & 35.56$\pm$1.92                  & 41.26$\pm$1.49                   & 40.36$\pm$1.73                  & 60.36$\pm$1.49                  & 59.10$\pm$1.70                  & 43.19$\pm$1.56                  & 42.69$\pm$1.44                  \\
                      & w GMix                 & 37.52$\pm$2.11                   & 36.26$\pm$2.04                  & 40.39$\pm$2.19                   & 40.02$\pm$2.11                  & 60.99$\pm$1.75                  & 60.36$\pm$1.59                  & 43.32$\pm$1.74                  & 42.79$\pm$1.96                  \\
                      & ours                   & \textbf{42.64$\pm$2.02}          & \textbf{41.27$\pm$1.65}         & \textbf{56.36$\pm$2.02}          & \textbf{55.25$\pm$1.75}         & \textbf{62.44$\pm$1.35}         & \textbf{61.66$\pm$1.29}         & \textbf{46.24$\pm$1.60}         & \textbf{44.54$\pm$1.62}         \\ \midrule
\multirow{4}{*}{10}   & SGC                    & 39.39$\pm$1.52                   & 38.52$\pm$1.11                  & 42.01$\pm$1.37                   & 41.45$\pm$1.32                  & 61.92$\pm$1.41                  & 61.42$\pm$1.72                  & 47.19$\pm$2.21                  & 46.36$\pm$2.01                  \\
                      & w GAug                 & 39.76$\pm$1.79                   & 38.62$\pm$1.56                  & 42.29$\pm$1.66                   & 41.66$\pm$1.73                  & 62.09$\pm$1.57                  & 61.69$\pm$1.63                  & 47.30$\pm$2.19                  & 46.62$\pm$1.94                  \\
                      & w GMix                 & 39.92$\pm$1.93                   & 39.36$\pm$1.76                  & 43.39$\pm$2.03                   & 42.91$\pm$1.97                  & 62.39$\pm$1.60                  & 62.02$\pm$1.49                  & 47.39$\pm$1.75                  & 46.92$\pm$1.66                  \\
                      & ours                   & \textbf{45.14$\pm$1.29}          & \textbf{43.69$\pm$1.10}         & \textbf{58.84$\pm$1.79}          & \textbf{57.53$\pm$1.56}         & \textbf{64.54$\pm$1.22}         & \textbf{64.16$\pm$1.20}         & \textbf{48.82$\pm$1.12}         & \textbf{47.26$\pm$1.19}         \\ \midrule
\multirow{4}{*}{15}   & SGC                    & 41.29$\pm$2.56                   & 40.76$\pm$2.35                  & 43.76$\pm$2.02                   & 42.66$\pm$2.43                  & 63.12$\pm$1.97                  & 62.39$\pm$1.74                  & 47.12$\pm$3.19                  & 45.26$\pm$3.05                  \\
                      & w GAug                 & 41.53$\pm$1.22                   & 40.99$\pm$1.60                  & 43.96$\pm$1.31                   & 42.96$\pm$1.22                  & 63.29$\pm$1.40                  & 62.90$\pm$1.45                  & 47.39$\pm$1.32                  & 45.69$\pm$1.63                  \\
                      & w GMix                 & 42.36$\pm$1.41                   & 41.26$\pm$2.73                  & 44.39$\pm$2.59                   & 43.20$\pm$2.44                  & 63.39$\pm$2.40                  & 63.09$\pm$2.37                  & 47.59$\pm$2.18                  & 45.92$\pm$2.10                  \\
                      & ours                   & \textbf{45.88$\pm$1.36}          & \textbf{44.10$\pm$1.22}         & \textbf{59.08$\pm$1.55}          & \textbf{55.96$\pm$1.50}         & \textbf{65.04$\pm$1.19}         & \textbf{64.43$\pm$1.26}         & \textbf{49.26$\pm$1.55}         & \textbf{47.70$\pm$1.36}         \\ \midrule
\multirow{4}{*}{20}   & SGC                    & 41.92$\pm$3.26                   & 41.16$\pm$2.72                  & 45.02$\pm$3.73                   & 44.66$\pm$3.60                  & 63.90$\pm$3.35                  & 63.19$\pm$2.66                  & 47.36$\pm$2.59                  & 45.62$\pm$2.23                  \\
                      & w GAug                 & 42.06$\pm$3.19                   & 41.60$\pm$2.74                  & 45.26$\pm$2.59                   & 44.99$\pm$2.73                  & 64.06$\pm$2.56                  & 63.42$\pm$2.70                  & 47.96$\pm$2.19                  & 45.99$\pm$2.31                  \\
                      & w GMix                 & 42.36$\pm$2.56                   & 41.99$\pm$2.40                  & 45.99$\pm$2.37                   & 45.26$\pm$2.42                  & 63.92$\pm$2.31                  & 63.29$\pm$2.56                  & 48.36$\pm$2.15                  & 47.92$\pm$2.26                  \\
                      & ours                   & \textbf{46.72$\pm$1.96}          & \textbf{45.65$\pm$1.66}         & \textbf{59.38$\pm$1.62}          & \textbf{58.25$\pm$1.60}         & \textbf{65.78$\pm$1.32}         & \textbf{65.42$\pm$1.26}         & \textbf{49.52$\pm$1.29}         & \textbf{47.88$\pm$1.26}         \\ \bottomrule
\end{tabular}%
}
\end{table*}
Based on the results, we observe that incorporating graph augmentation techniques can result in slight performance improvements for the SGC model. This is attributed to the ability of graph augmentation to facilitate the learning of high-quality node representations by the model.

\subsection{Model Performance with Different Graph Encoders}
To further validate the flexibility of our proposed model, we replace the graph backbone with GCN \cite{kipf2016semi}, GAT \cite{velivckovic2017graph}, SAGE \cite{hamilton2017inductive}, and GraphGPS \cite{rampavsek2022recipe} under the 5 way 5 shot setting. The results of these experiments are presented in Table \ref{res_backbone}. According to the results, we find that our proposed method, even when equipped with different graph encoders, still achieves excellent performance across various datasets under different experimental settings, providing strong evidence of its effectiveness.

\begin{table*}[ht]
\centering

\caption{Results (\%) of our model on the datasets under various backbones.}
%\tiny
\label{res_backbone}
\resizebox{\textwidth}{!}{%
\begin{tabular}{@{}c|c|cccccccc@{}}
\toprule
\multirow{2}{*}{Task} & \multirow{2}{*}{Backbone} & \multicolumn{2}{c}{Amazon-Clothing}                        & \multicolumn{2}{c}{CoraFull}                        & \multicolumn{2}{c}{Amazon-Electronics}                    & \multicolumn{2}{c}{DBLP}                           \\ \cmidrule(l){3-10} 
                      &                           & Acc                      & F1                       & Acc                      & F1                       & Acc                      & F1                      & Acc                      & F1                      \\ \midrule
\multirow{5}{*}{5}    & GCN                       & 81.76$\pm$1.39                    & 81.29$\pm$1.95                    & 65.96$\pm$1.66                    & 65.25$\pm$2.02                    & \textbf{67.96$\pm$2.11}           & \textbf{66.82$\pm$1.96}          & 75.52$\pm$2.32                    & 74.75$\pm$2.30                   \\
                      & GAT                       & 80.19$\pm$2.21                    & 79.59$\pm$2.02                    & 63.99$\pm$1.97                    & 63.36$\pm$1.73                    & 66.75$\pm$1.66                    & 65.32$\pm$1.55                   & 73.96$\pm$1.50                    & 73.96$\pm$1.45                   \\
                      & SAGE                      & \textbf{82.92$\pm$1.70}           & \textbf{82.52$\pm$1.49}           & \textbf{66.82$\pm$1.53}           & \textbf{66.36$\pm$1.39}           & 67.10$\pm$1.75                    & 66.16$\pm$1.50                   & 75.39$\pm$2.22                    & 74.95$\pm$1.92                   \\
                      & GraphGPS                  & 80.25$\pm$1.99                    & 78.26$\pm$1.97                    & 64.39$\pm$1.85                    & 63.95$\pm$1.82                    & 66.19$\pm$1.80                    & 65.29$\pm$2.36                   & 73.29$\pm$2.39                    & 72.72$\pm$2.52                   \\
                      & SGC (ours)                & 82.80$\pm$2.19                    & 82.49$\pm$2.26                    & 66.34$\pm$2.28                    & 65.70$\pm$2.52                    & 67.30$\pm$2.59                    & 66.30$\pm$2.32                   & \textbf{75.88$\pm$2.21}           & \textbf{75.05$\pm$2.22}          \\ \midrule
\multirow{5}{*}{10}   & GCN                       & 82.56$\pm$2.36                    & 82.29$\pm$2.30                    & \textbf{72.20$\pm$2.15}           & \textbf{71.35$\pm$2.45}           & 69.76$\pm$2.29                    & 69.22$\pm$2.26                   & 75.39$\pm$2.17                    & 74.62$\pm$2.79                   \\
                      & GAT                       & 81.92$\pm$2.36                    & 80.96$\pm$2.66                    & 70.92$\pm$1.80                    & 70.39$\pm$1.77                    & 68.15$\pm$2.16                    & 67.29$\pm$2.30                   & 74.99$\pm$2.22                    & 74.29$\pm$2.15                   \\
                      & SAGE                      & 83.02$\pm$1.73                    & 82.56$\pm$1.79                    & 71.96$\pm$2.32                    & 71.52$\pm$2.25                    & 70.26$\pm$2.26                    & 70.15$\pm$2.21                   & 76.32$\pm$2.46                    & 75.32$\pm$2.39                   \\
                      & GraphGPS                  & 81.26$\pm$2.11                    & 80.76$\pm$2.23                    & 70.15$\pm$2.25                    & 69.69$\pm$2.76                    & 67.92$\pm$2.82                    & 66.95$\pm$2.37                   & 74.25$\pm$2.29                    & 74.12$\pm$2.46                   \\
                      & SGC (ours)                & \textbf{83.46$\pm$1.66}           & \textbf{82.88$\pm$1.35}           & 71.72$\pm$1.95                    & 71.15$\pm$1.76                    & \textbf{70.76$\pm$1.32}           & \textbf{70.05$\pm$1.90}          & \textbf{76.64$\pm$1.56}           & \textbf{75.77$\pm$1.38}          \\ \midrule
\multirow{2}{*}{Task} & \multirow{2}{*}{Model}    & \multicolumn{2}{c}{Amazon-Clothing$\rightarrow$CoraFull} & \multicolumn{2}{c}{CoraFull$\rightarrow$Amazon-Clothing} & \multicolumn{2}{c}{Amazon-Electronics$\rightarrow$DBLP} & \multicolumn{2}{c}{DBLP$\rightarrow$Amazon-Electronics} \\ \cmidrule(l){3-10} 
                      &                           & Acc                      & F1                       & Acc                      & F1                       & Acc                      & F1                      & Acc                      & F1                      \\ \midrule
\multirow{5}{*}{5}    & GCN                       & 42.16$\pm$1.88                    & 41.75$\pm$1.82                    & 55.79$\pm$1.81                    & 54.66$\pm$1.85                    & 62.19$\pm$1.39                    & 60.99$\pm$1.22                   & 46.09$\pm$1.26                    & 45.69$\pm$1.21                   \\
                      & GAT                       & 40.25$\pm$1.29                    & 40.02$\pm$1.26                    & 53.32$\pm$1.22                    & 52.12$\pm$1.34                    & 61.02$\pm$1.36                    & 60.19$\pm$1.42                   & 45.62$\pm$1.58                    & 45.19$\pm$1.52                   \\
                      & SAGE                      & 41.99$\pm$1.57                    & 40.95$\pm$1.59                    & 55.96$\pm$1.64                    & 55.29$\pm$1.43                    & \textbf{62.92$\pm$1.41}           & \textbf{62.29$\pm$1.30}          & 47.19$\pm$1.36                    & 45.20$\pm$1.33                   \\
                      & GraphGPS                  & 39.62$\pm$1.49                    & 38.66$\pm$1.52                    & 52.29$\pm$1.55                    & 51.96$\pm$1.66                    & 60.72$\pm$1.60                    & 59.79$\pm$1.53                   & 45.02$\pm$1.42                    & 44.16$\pm$1.51                   \\
                      & SGC (ours)                & \textbf{42.64$\pm$1.20}           & \textbf{41.27$\pm$1.22}           & \textbf{56.36$\pm$1.39}           & \textbf{55.25$\pm$1.30}           & 62.44$\pm$1.55                    & 61.66$\pm$1.26                   & 46.24$\pm$1.22                    & 44.54$\pm$1.66                   \\ \midrule
\multirow{5}{*}{10}   & GCN                       & 43.12$\pm$1.24                    & 42.26$\pm$1.26                    & 57.65$\pm$1.32                    & 57.16$\pm$1.39                    & 63.25$\pm$1.42                    & 62.35$\pm$1.49                   & 47.22$\pm$1.55                    & 46.29$\pm$2.12                   \\
                      & GAT                       & 43.19$\pm$2.12                    & 42.59$\pm$2.19                    & 56.99$\pm$2.22                    & 56.36$\pm$2.55                    & 62.39$\pm$2.36                    & 61.96$\pm$1.91                   & 46.29$\pm$2.16                    & 45.56$\pm$2.59                   \\
                      & SAGE                      & 44.66$\pm$2.66                    & 44.25$\pm$2.75                    & 58.16$\pm$2.30                    & 57.25$\pm$2.36                    & 63.92$\pm$2.15                    & 62.92$\pm$2.50                   & 48.09$\pm$1.72                    & 47.02$\pm$1.76                   \\
                      & GraphGPS                  & 42.26$\pm$1.79                    & 42.09$\pm$1.92                    & 55.26$\pm$1.22                    & 55.12$\pm$2.05                    & 61.52$\pm$2.17                    & 60.92$\pm$2.09                   & 46.25$\pm$2.01                    & 45.29$\pm$2.06                   \\
                      & SGC (ours)                & \textbf{45.14$\pm$2.19}           & \textbf{43.69$\pm$2.22}           & \textbf{58.84$\pm$2.39}           & \textbf{57.53$\pm$2.26}           & \textbf{64.54$\pm$1.79}           & \textbf{64.16$\pm$1.86}          & \textbf{48.82$\pm$1.79}           & \textbf{47.22$\pm$1.66}          \\ \bottomrule
\end{tabular} %
}
\end{table*}

\subsection{Model Performance for Few-shot Graph Classification}
In this section, we explore the application of our method to few-shot graph classification tasks. By utilizing graph pooling operations to obtain graph-level features, extending our model to downstream graph-level tasks is straightforward. To support this, we select several representative datasets Letter-high, ENZYMES, TRIANGLES, and Reddit, which are widely used for few-shot graph classification. We provide the statistics of evaluated datasets in Table \ref{dataset_graph}. Detailed descriptions of these datasets are provided below. 

\noindent $\bullet$ \textbf{Letter-high} contains graphs representing the English alphabet, with each label corresponding to a specific letter type.

\noindent $\bullet$ \textbf{ENZYMES} is a protein tertiary structure dataset composed of enzymes from the BRENDA database, with each class corresponding to a top-level enzyme.

\noindent $\bullet$ \textbf{TRIANGLES} consists of graphs, where the category is determined by the number of triangles (3-cliques) present in each graph.

\noindent $\bullet$ \textbf{Reddit} contains graphs representing threads, where each node represents a user, and different graph labels correspond to different types of forums.

\begin{table}[ht]
\centering
%\tiny

\caption{Statistics of the evaluated datasets.}
\label{dataset_graph}
%\resizebox{0.7\textwidth}{!}{%
\begin{tabular}{@{}c|ccccc@{}}
\toprule
Dataset                          & \# Graphs & \# Nodes & \# Edges & \# Classes & \# Novel\\ \midrule
Letter-high & 2,250     & 4.67     & 4.50     & 15         & 4       \\
ENZYMES     & 600       & 32.63    & 62.14    & 6          & 2        \\
TRIANGLES                        & 2,000     & 20.85    & 35.50    & 10         & 3        \\
Reddit  & 1,111     & 391.41   & 456.89   & 11         & 4        \\ \bottomrule
\end{tabular}%
%}
\end{table}

\begin{table*}[ht]

\caption{Results of different models on few-shot graph classification tasks.}
\label{res}
\begin{tabular}{@{}c|cccccccc@{}}
\toprule
\multirow{2}{*}{Model} & \multicolumn{2}{c}{Letter-high} & \multicolumn{2}{c}{ENZYMES}     & \multicolumn{2}{c}{TRIANGLES}   & \multicolumn{2}{c}{Reddit}      \\ \cmidrule(l){2-9} 
        & 5-shot & 10-shot & 5-shot & 10-shot & 5-shot & 10-shot & 5-shot & 10-shot \\ \midrule
GSM     & 69.91$\pm$5.90  & 73.28$\pm$3.64   & 55.42$\pm$5.74  & 60.64$\pm$3.84   & 71.40$\pm$4.34  & 75.60$\pm$3.67   & 41.59$\pm$4.12  & 45.67$\pm$3.68   \\
AS-MAML & 69.44$\pm$0.75  & 75.93$\pm$0.53   & 49.83$\pm$1.12  & 52.30$\pm$1.43   & 78.42$\pm$0.67  & 80.39$\pm$0.56   & 36.96$\pm$0.74  & 41.47$\pm$0.83   \\
FAITH   & 71.55$\pm$3.58  & 76.65$\pm$3.26   & 57.89$\pm$4.65  & 62.16$\pm$4.11   & 79.59$\pm$4.05  & 80.79$\pm$3.53   & 42.71$\pm$4.18  & 46.63$\pm$4.01   \\
SMART   & 74.17$\pm$2.75       &  76.89$\pm$1.55       &  59.80$\pm$3.39      &   65.11$\pm$2.70      & 79.39$\pm$2.45       & 80.43$\pm$2.12        &  43.83$\pm$2.21      & 47.75$\pm$2.77        \\
Ours                   & \textbf{76.56$\pm$1.96} & \textbf{79.22$\pm$2.32} & \textbf{61.35$\pm$3.75} & \textbf{67.19$\pm$2.89} & \textbf{81.22$\pm$2.66} & \textbf{82.56$\pm$2.75} & \textbf{45.72$\pm$2.39} & \textbf{49.26$\pm$2.82} \\ \bottomrule
\end{tabular}
\end{table*}

We choose several representative few-shot graph classification models, GSM \cite{chauhan2020few}, AS-MAML \cite{ma2020adaptive}, FAITH \cite{wang2022faith}, and SMART \cite{liu2024simple}, for comparison. The detailed descriptions of these models are presented below. 

\noindent $\bullet$ \textbf{GSM} \cite{chauhan2020few}: It generates a set of superclasses through graph spectral metrics and constructs corresponding super-graphs to model the relationships between the classes.

\noindent $\bullet$ \textbf{AS-MAML} \cite{ma2020adaptive}: It directly combines GNN and MAML to quickly adapt to unseen test graphs, utilizing a step controller to enhance the robustness of the meta-trainer.

\noindent $\bullet$ \textbf{FAITH} \cite{wang2022faith}: It captures task relevance by constructing hierarchical graphs of varying granularity, thereby enhancing the model's adaptability to unseen new classes.

\noindent $\bullet$ \textbf{SMART} \cite{liu2024simple}: It replaces the complex meta-learning training paradigm with a simpler transfer learning approach, utilizing graph contrastive learning and prompt learning to enhance the model's representation extraction capability and learning efficiency.

We present the results of our model and these baselines in the Table \ref{res}. According to the results, we can find that our model significantly surpasses other baseline models across multiple datasets under various experimental settings, clearly demonstrating the superiority and adaptability of our approach.

\subsection{Performance Varies with Mixup Parameters}
In this section, we investigate the sensitivity of the performance of our proposed model to the parameters of the Beta distribution used in the developed mixing strategy. We present how the performance of our model varies with the Beta distribution parameters, $\alpha$ and $\beta$, across different datasets under the 5-way 5-shot 5 tasks few-shot experimental settings. For simplicity, we always keep $\alpha$ and $\beta$ equal. As shown in Fig. \ref{mixup_hyper}, we observe that our model exhibits good robustness concerning this parameter. As the parameters change, the model performance maintains a stable trend.

\begin{figure*}

    \centering
    \subfigure[in-domain]{\includegraphics[width=0.45\linewidth]{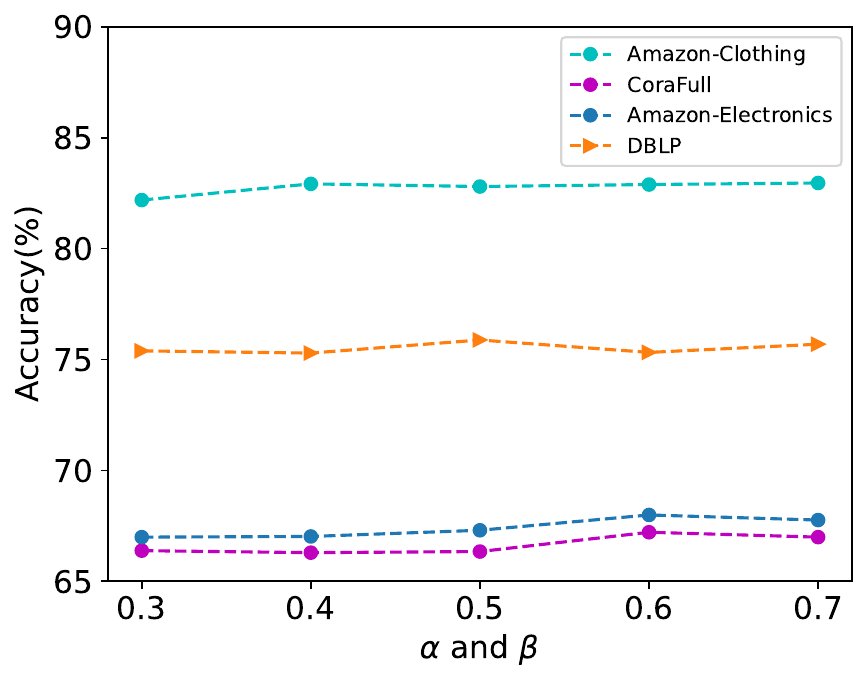}}
    \subfigure[cross-domain]{\includegraphics[width=0.45\linewidth]{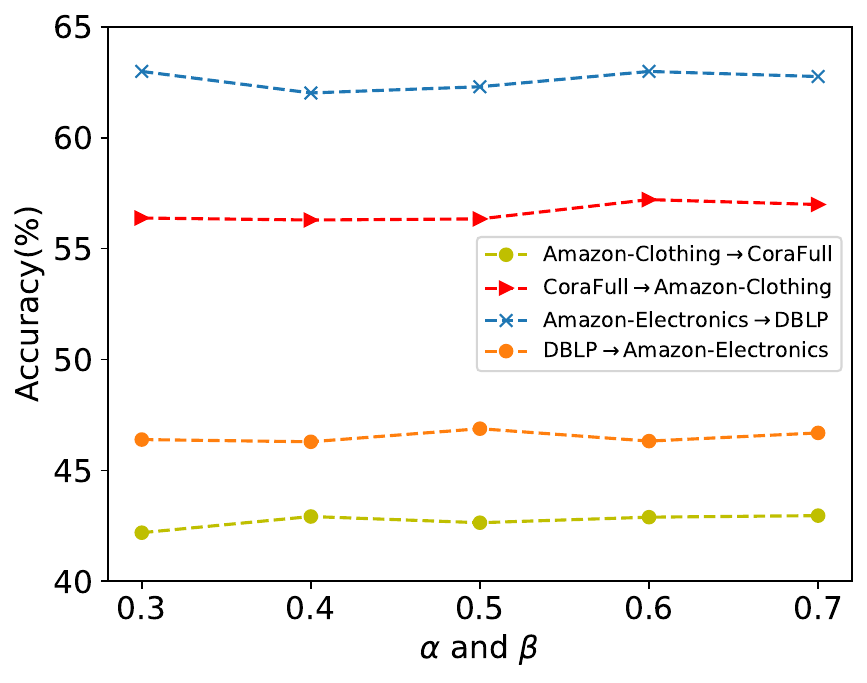}}
    \caption{Model performance varies with the values of the mixup hyperparameters $\alpha$ and $\beta$.}
    \label{mixup_hyper}
\end{figure*}

\subsection{Exploring Model Generalization Gap}
\begin{figure*}[ht]

    \centering
    \subfigure[Amazon-Clothing]{\includegraphics[width=0.49\textwidth]{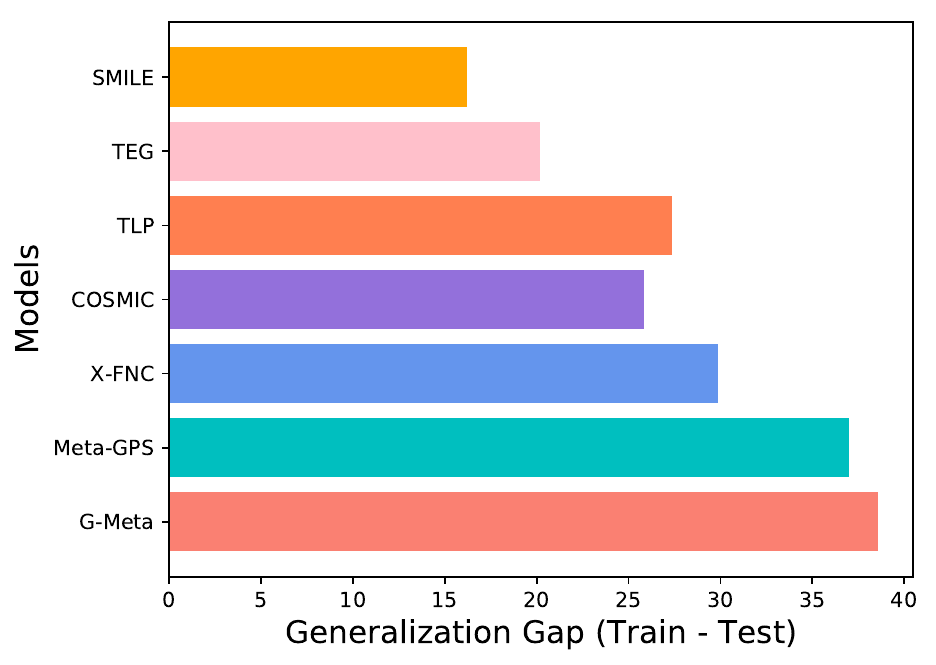}}
    \subfigure[Amazon-Clothing$\rightarrow$CoraFull]{\includegraphics[width=0.49\textwidth]{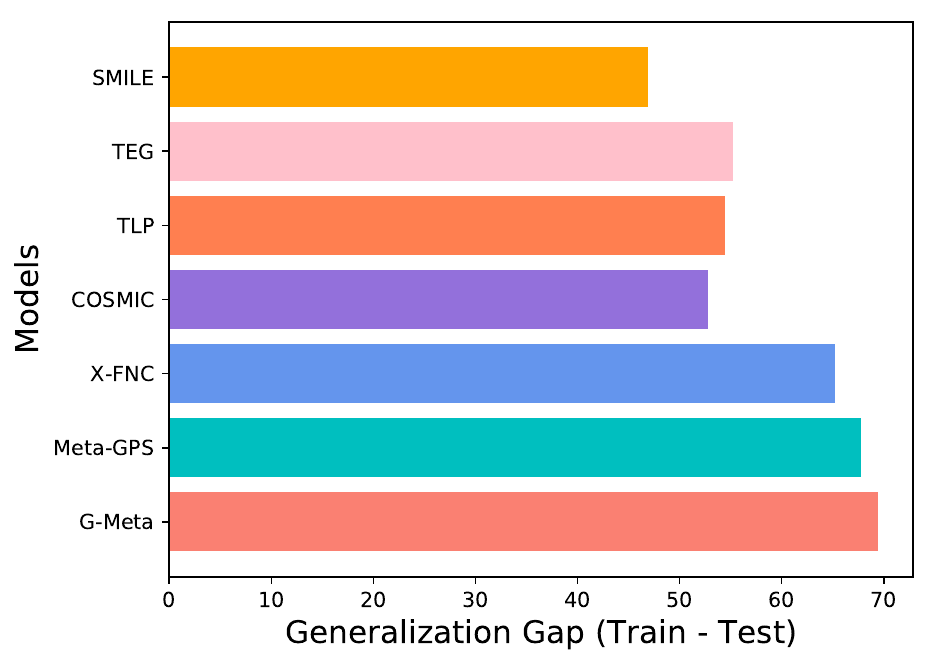}}
    \caption{(a) Generalization gap over several methods on the Amazon-Clothing dataset under the 5-way 5-shot 5 tasks setting. (b) Generalization gap over several methods on the Amazon-Clothing dataset under the 5-way 5-shot 5 tasks setting.}
    \label{gap_in}
\end{figure*}

Moreover, we further investigate whether SMILE can improve its generalization capability by reducing the generalization gap, where the generalization gap is empirically defined as the disparity between the model's accuracy on the meta-training tasks and its accuracy on the meta-testing tasks. Fig. \ref{gap_in} illustrates the generalization gap induced by different models under the 5-way 5-shot few-shot setting, including both in-domain and cross-domain settings. Upon comparing the disparities depicted in Fig. \ref{gap_in} (a) and (b), it is evident that the discrepancy between the training and testing accuracies when employing our method consistently remains smaller than that of other methods. These results empirically support our theoretical findings, showing that, compared to standard training without dual-levl mixup, SMILE consistently exhibits a smaller generalization gap with high probability. This further confirms the effectiveness of our proposed method under both in-domain and cross-domain settings.

\section{Visualization Study}
\label{visualization_study}
\begin{figure*}[ht]

    \centering
    \subfigure[within-task mixup]{\includegraphics[width=0.52\textwidth]{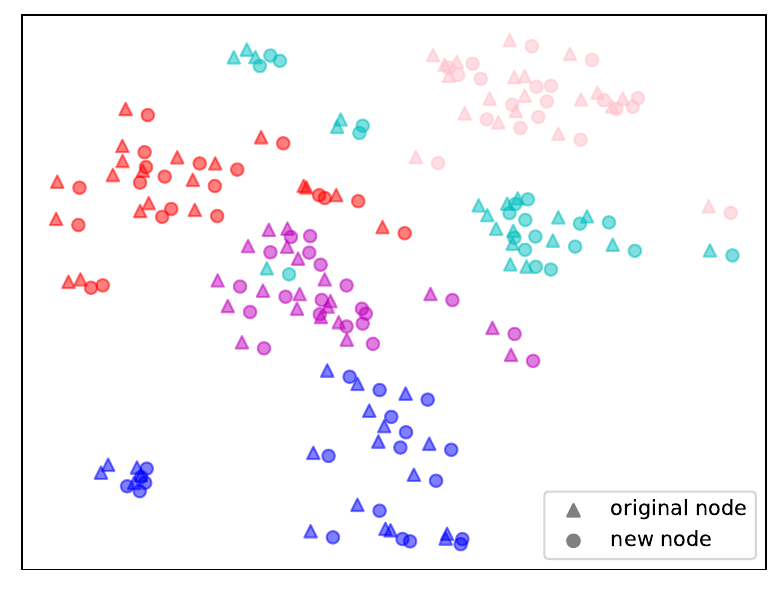}}
    \subfigure[across-task mixup]{\includegraphics[width=0.505\textwidth]{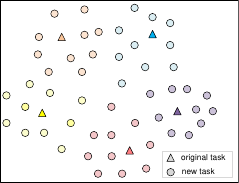}}
    \caption{Visualization of the dual-level mixup strategies. In (a), the original nodes in each task are represented by triangles, while the generated nodes are represented by circles, with colors indicating the corresponding classes. In (b), the original tasks are represented by triangles, the generated tasks are represented by circles, and the colors indicate the most similar original tasks.}
    \label{Vis}
\end{figure*}
To visually present the introduced dual-level mixup strategy, we leverage t-SNE \cite{van2008visualizing} to visualize the results of dual-level mixup on the Amazon-clothing dataset under the 5-way 5-shot with 5 tasks few-shot setting, as shown in Fig. \ref{Vis}. Specifically, in the within-task mixup, we randomly select one task consisting of support and query sets. In the across-task, we interpolate 50 tasks, where the task embeddings are the average of the contained node embeddings. According to Fig. \ref{Vis}, we observe that the interpolated nodes within each task and the interpolated tasks generated by SMILE indeed densify the node and task distributions, thereby enhancing the model generalization capability.

% \section{Limitation}
% \label{limitation}
% Although our proposed method has achieved outstanding in both in-domain and cross-domain few-shot node classification tasks, a potential limitation is that our model primarily focuses on classification problems, making it difficult to directly apply to link prediction or regression tasks. In future work, further enhancing the adaptability of our model to extend to more scenarios would be highly valuable.

% \section{Broad Impacts}
% \label{impact}
% This work aims to develop a simple yet effective approach for graph few-shot learning with fewer tasks. Our approach is potentially applicable to few-shot learning not just within graph domains, but more broadly across other domains as well. Furthermore, our work does not involve ethical issues and may have many potential societal consequences, but we do not feel that they need to be specifically highlighted here.
